# Supplementary material for: Faster and Non-ergodic O(1/K) Stochastic Alternating Direction Method of Multipliers
Source: arXiv:1704.06793 source file (2017-04-22)
Supplement: Supplementary file 1 [file appendix.tex]

\section*{Supplementary Materials}

\section*{Outline of Proof}
Below is the outline of our proof. We will ignore the subscript
$s$ if $s$ is fixed in the equation, since some analysis are in a single epoch. \\\\ 
Step: 1 
\\Through the optimal solution of $\x_1$, we can obtain:
\begin{eqnarray}\label{step1}
&&F_1(\x^{k+1}_1)\\
&\leq& (1-\theta_1-\theta_2)F_1(\x^k_1)+ \theta_2 F_1(\tx_1)+\theta_1 F_1(\x_1^*)\notag\\
&&-\langle \A_1^T\blam(\x^{k+1}_1,\y^k_2)  ,\x^{k+1}_1-(1-\theta_1-\theta_2)\x^k_1-\theta_2 \tx_1-\theta_1\x_1^*  \rangle +\frac{L_1}{2}\|\x^{k+1}_1-\y^k_1  \|^2 \notag\\
&&  - \left\langle  \x^{k+1}_1-\y^{k}_1, \x^{k+1}_1-(1-\theta_1-\theta_2)\x^k_1-\theta_2\tx_1-\theta_1\x^*\right\rangle_{\left(L_1+\frac{\beta \| \A_1^T \A_1\|}{\theta_1}\right)\I-\frac{\beta\A_1^T\A_1}{\theta_1} },\notag
\end{eqnarray}
where we set $\blam(\x_1,\x_2) = \frac{\beta}{\theta_1}\left(\A_1 \x_1 +\A_2 \x_2-\b\right)+\olam^k$.\\\\ 
Step: 2\\ 
Through the optimal solution of $\x_2$, and using the technique that is mentioned in Section 3.2 of our paper,  we can obtain:
\begin{eqnarray}\label{step2}
&&\E_{i_{k}}F_2(\x^{k+1}_2)\notag\\
&\leq&- \E_{i_{k}}\left\langle  \A_2^T\blam(\x^{k+1}_1,\y^k_2)+  \left(\alpha L_2+\frac{\beta\| \A_2^T \A_2\|}{\theta_1} \right)\left(\x^{k+1}_2-\y^{k}_2\right) ,  \x^{k+1}_2 -\theta_2\tx_2\right  \rangle\notag\\
&&- \E_{i_{k}}\left\langle  \A_2^T\blam(\x^{k+1}_1,\y^k_2)+  \left(\alpha L_2+\frac{\beta\| \A_2^T \A_2\|}{\theta_1} \right)\left(\x^{k+1}_2-\y^{k}_2\right) ,  - (1-\theta_2-\theta_1)\x^k_{2}-\theta_1\x_2^* \right  \rangle\notag\\
&&+(1-\theta_2-\theta_1)F_2(\x^{k}_2) +\theta_1F_2(\x_2^*) +\theta_2 F_2(\tx_2) +\E_{i_{k}}\left( \frac{(1+\frac{1}{b\theta_2})L_2}{2}\| \x^{k+1}_2-\y^k_2\|^2 \right),
\end{eqnarray}
where $\E_{i_k}$ indicates that the expectation is  taken over the random choice of $i_{k,s}$,  under the condition that $\y_2^k$, $\tx_2$ and $\x^k_2$ (the  randomness in the first $sm+k$ iterations are fixed) are known.\\\\
Step: 3\\
We consider the multiplier. Setting $\hlam^{k} = \tlam^{k} +\frac{\beta(1-\theta_1)}{\theta_1}(\A_1\x^{k}_1+\A_2\x^{k}_2-\b)$, it has the following properties:
\begin{eqnarray}
\hlam^{k+1}&=&\blam(\x^{k+1}_1,\x^{k+1}_2),\\
\hlam^{k+1}-\hlam^{k}&=&\frac{\beta A_1}{\theta_1}\left(\x^{k+1}_1-(1-\theta_1)\x_1^{k}-\theta_1\x_1^* +\theta_2(\x^k_1-\tx_1)\right),\notag\\
&&+ \frac{\beta A_2}{\theta_1}\left(\x^{k+1}_2-(1-\theta_1)\x_2^{k}-\theta_1\x_2^* +\theta_2(\x^k_2-\tx_2) \right),\\
\hlam^0_{s} &=&\hlam^m_{s-1}.
\end{eqnarray}\\
Step: 4\\
Adding Eq.~\eqref{step1} and Eq.~\eqref{step2}, and simplifying the result, we obtain Lemma $1$:
\begin{eqnarray}\label{step4}
&& \!\!\!\!\!\!\!\E_{i_k}\left(L(\x^{k+1}_1,\x^{k+1}_2,\olam^*)\right) - \theta_2 L(\tx_1,\tx_2,\olam^*) -(1-\theta_2 - \theta_1)L(\x^{k}_1,\x^{k}_2,\olam^*)\\
&\leq&  \frac{\theta_1}{2\beta}\left(\|\hlam^k-\olam^*\|^2- \E_{i_k}\|\hlam^{k+1}-\olam^*\|^2 \right)\notag\\
&&+\frac{1}{2}\|\y_1^{k}-(1-\theta_1-\theta_2)\x_1^{k}-\theta_2\tx_1-\theta_1\x_1^*\|^2_{\left(L_1+\frac{\beta\| \A_1^T \A_1\|}{\theta_1}\right)\I-\frac{\beta\A_1^T\A_1}{\theta_1} }\notag\\
&&-\frac{1}{2}\E_{i_k}\left(\|\x^{k+1}_1-(1-\theta_1-\theta_2)\x_1^{k}-\theta_2\tx_1-\theta_1\x_1^*\|^2_{\left(L_1+\frac{\beta\| \A_1^T \A_1\|}{\theta_1}\right)\I-\frac{\beta\A_1^T\A_1}{\theta_1} }\right)\notag\\
&&+ \frac{1}{2} \|\y_2^{k}-(1-\theta_1-\theta_2)\x^k_2-\theta_2\tx_2-\theta_1\x_2^*\|^2_{\left(\alpha L_2+\frac{\beta\| \A_2^T \A_2\|}{\theta_1}\right)\I}\notag\\
&&-\frac{1}{2} \E_{i_k} \left(\|\x_2^{k+1}-(1-\theta_1-\theta_2)\x^k_2-\theta_2\tx_2-\theta_1\x_2^*\|^2_{\left(\alpha L_2+\frac{\beta\| \A_2^T \A_2\|}{\theta_1}\right)\I}\right)\notag,
\end{eqnarray}
where we define $L(\x_1,\x_2,\olam) =  F_1(\x_1) - F_1(\x^*_1)+ F_2(\x_2)-F_2(\x^*_2) + \langle \olam, \A_1\x_1+\A_2\x_2-\b  \rangle$.\\\\
Step: 5\\
In step $5$, we will first divide $\theta_{1}$ on both side of Eq.~\eqref{step4} and then  summing it with $k$ from $0$ to $m-1$. Then after some simplifying, we can obtain
\begin{eqnarray}\label{step5}
&&\frac{1}{\theta_{1,s}}\E\left(L(\x^{m}_s,\olam^*)-L(\x^*,\olam^*)\right)+ \frac{\theta_{2}+\theta_{1,s}}{\theta_{1,s}}\sum_{k=1}^{m-1} \E\left(L(\x^{k}_s,\olam^*)-L(\x^*,\olam^*)\right)\notag\\
&\leq&   \frac{1}{\theta_{1,s-1}}\E\left(L(\x^{m}_{s-1},\olam^*)-L(\x^*,\olam^*)\right)+ \frac{\theta_2+\theta_{1,{s-1}}}{\theta_{1,s-1}}\sum_{k=1}^{m-1}\E\left(L(\x^{k}_{s-1},\olam^*)-L(\x^*,\olam^*)\right)\notag\\
&&+\frac{1}{2}\E\| \frac{ \y^{0}_{s,1}-\theta_2\tx_{s,1}-(1-\theta_{1,s}-\theta_{2})\x^{0}_{s,1}}{\theta_{1,s}}-\x^*_1   \|^2_{\left(\theta_{1,s}L_1+\| \A_1^T \A_1\|\right)\I-\A_1^T\A_1}\notag\\
&&-\frac{1}{2}\E\| \frac{ \x^{m}_{s,1}-\theta_2\tx_{s,1}-(1-\theta_{1,s}-\theta_{2})\x^{m-1}_{s,1}}{\theta_{1,s}}-\x^*_1   \|^2_{\left(\theta_{1,s}L_1+\| \A_1^T \A_1\|\right)\I-\A_1^T\A_1}\notag\\
&&+\frac{1}{2}\E\| \frac{ \y^{0}_{s,2}-\theta_2\tx_{s,2}-(1-\theta_{1,s}-\theta_{2})\x^{0}_{s,2}}{\theta_{1,s}}-\x^*_2   \|^2_{\left(\alpha \theta_{1,s}L_2+\| \A_2^T \A_2\|\right)\I}\notag\\
&&-\frac{1}{2}\E\| \frac{ \x^{m}_{s,2}-\theta_2\tx_{s,2}-(1-\theta_{1,s}-\theta_{2})\x^{m-1}_{s,2}}{\theta_{1,s}}-\x^*_2   \|^2_{\left(\alpha \theta_{1,s}L_2+\| \A_2^T \A_2\|\right)\I}\notag\\
&& +\frac{1}{2\beta}\left(\E\|\hlam^0_s-\olam^*\|^2- \E\left[\|\hlam^{m}_s-\olam^*\|^2\right] \right),
\end{eqnarray}
where we denote $L(\x^k_s,\olam^*)$ and $L(\tx_s,\olam^*)$ to denote $L(\x^k_{s,1},  \x^k_{s,2},\olam^*)$ and $L(\tx_{s,1},\tx_{s,2}, \olam^*)$, respectively. Note that diving $\theta_{1}$~(not $\theta_{1}^2$ ) on both side of Eq.~\eqref{step4} enables us to achieve the non-ergodic $O(1/S)$ result.\\\\
Step: 6\\
Summing Eq.~\eqref{step5} with $s$ from $0$ to $S-1$, and simplifying the result, we obtain Theorem 1:
\begin{eqnarray}
&&\frac{1}{2\beta}\E\|\frac{\beta m}{\theta_{1,{S}}}\left(\A\hat{\x}_{S}\!-\!\b\right)-\frac{\beta(m\!-\!1)\theta_{2}}{\theta_{1,{0}}}\left(\A\x^0_{0}-\b\right) +\tlam^0_0-\olam^*\! \|^ \\
&&+\frac{m}{\theta_{1,{S}}}\E\left(F(\hat{\x}_{S})-F(\x^*)  +\langle \olam^*, \A\hat{\x}_S -\b\rangle\right) \notag\\
&\leq& C_3\left(F(\x_{0}^0)-F(\x^*)  +\langle \olam^*, \A\x^0_0 -\b\rangle\right)+\frac{1}{2\beta}\|\tlam^0_0 +\frac{\beta(1-\theta_{1,{0}})}{\theta_{1,{0}}}(\A\x_0^0-\b) -\olam^*  \|^2\notag\\
&&+\frac{1}{2}\|\x^0_{0,1}-\x^*_1   \|^2_{\left(\theta_{1,0}L_1+\| \A_1^T \A_1\|\right)\I-\A_1^T\A_1}+\frac{1}{2}\| \x^0_{0,2}-\x^*_2  \|^2_{\left((1+\frac{1}{b\theta_2}) \theta_{1,0}L_2+\| \A_2^T \A_2\|\right)\I},\notag
\end{eqnarray}
where $C_3= \frac{1-\theta_{1,0}+(m-1)\theta_2}{\theta_{1,0}}$.\\\\
Step: 7\\
We prove Corollary 1:
\begin{eqnarray}
\E|F(\hat{\x}_{S})-F(\x^*)| &\leq& O(\frac{1}{S}),\notag\\ 
\E\| \A\hat{\x}_{S}-\b\| &\leq& O(\frac{1}{S}).
\end{eqnarray}

\section*{Proofs}
\bfseries  Proof of Eq.~(15) in the paper. \mdseries 
For completeness, we first include the proof of Eq.~($15$) in the paper. It is taken from~\cite{Katyusha, SVRG}.
\begin{eqnarray}\label{boundd}
&& \E_{i_k}\left(\|\nabla f_2(\y_2^k) - \tna f_2(\y_2^k)\|^2\right)\notag\\
&=& \E_{i_k} \left(\| \frac{1}{b}\sum_{i_{k,s}\in \mathcal{I}_{(k,s)}}\left(\nabla f_{2,i_{k,s}}(\y_2^k) - \nabla f_{2,i_{k,s}}(\tx_2) + \nabla f_2(\tx_2) - \nabla f_2(\y_2^k)\right)\|^2 \right)\notag\\ 
&\overset{a}=& \frac{1}{b} \E_{i_k} \left[\|\left(\nabla f_{2,i(k)}(\y^k_2)-  \nabla f_{2,i(k)}(\tx_2)\right) - \left(\nabla f_2(\y^k_2)-\nabla  f_2(\tx_2)\right)\|^2 \right]\notag\\
&\overset{b}\leq&\frac{1}{b} \E_{i_k} \left(\|\nabla f_{2,i(k)}(\y^k_2)- \nabla f_{2,i(k)}(\tx_2)\|^2\right)\notag\\
&\leq& \frac{2L_2}{b}  \E_{i_k} \left[ f_{2,i(k)}(\tx_2) -  f_{2,i(k)}(\y^k_2) -   \langle \nabla  f_{2,i(k)}(\y^k_2), \tx_2-\y^k_2  \rangle \right]\notag\\
&=& \frac{2L_2}{b} \left[ f_2(\tx_2) -  f_2(\y^k_2) -   \langle \nabla  f_2(\y^k_2), \tx_2-\y^k_2  \rangle \right],
\end{eqnarray}
where $\E_{i_k}$ indicates that the expectation is  taken over the random choice of $i_{k,s}$,  under the condition that $\y_2^k$, $\tx_2$ and $\x^k_2$ are known, in equality $\overset{a}=$, we denote $i(k)$ as a random sample over the training data, this equality is obtained since each $i_{k,s}$ is independent; the inequality $\overset{b}\leq$ uses the property that $\E\|\xi-\E(\xi)\|^2=\E\|\xi\|^2-\|\E\xi\|^2\leq \E\|\xi\|^2$.
\\\\
\bfseries  Proof of Step 1: \mdseries 

Set $\blam(\x_1,\x_2) = \frac{\beta}{\theta_1}\left(\A_1 \x_1 +\A_2 \x_2-\b\right)+\olam^k$. For the optimal solution of $\x_1$, we have
\begin{eqnarray}\label{first}
\left(L_1+\frac{\beta \| \A_1^T \A_1\|}{\theta_1} \right) \left(\x^{k+1}_1-\y^{k}_1\right) + \nabla f_1(\y^k_1) +\A_1^T\blam(\y^k_1,\y^k_2) \in -\partial h_1(\x^{k+1}_1).
\end{eqnarray} 
Since $f_1$ have Lipschitz continuous gradients, we have
\begin{eqnarray}
f_1(\x^{k+1}_1) &\leq& f_1(\y^{k}_1) + \langle \nabla f_1(\y^{k}_1),  \x^{k+1}_1 -\y^{k}_1 \rangle +\frac{L_1}{2}\| \x^{k+1}_1 -\y^{k}_1  \|^2\\
&\overset{a}\leq& f_1(\uu_1) + \langle \nabla f_1(\y^{k}_1),  \x^{k+1}_1 -\uu_1 \rangle + \frac{L_1}{2}\| \x^{k+1}_1 -\y^{k}_1  \|^2 \notag\\
&\overset{b}\leq& f_1(\uu_1) - \langle \partial h_1(\x^{k+1}_1)  , \x^{k+1}_1-\uu_1\rangle-\langle\A_1^T\blam(\y^k_1,\y^k_2)  ,\x^{k+1}_1-\uu_1 \rangle\notag\\
&&  -\left(L_1+\frac{\beta \| \A_1^T \A_1\|}{\theta_1}\right) \langle  \x^{k+1}_1-\y^{k}_1, \x^{k+1}_1-\uu_1\rangle+\frac{L_1}{2}\| \x^{k+1}_1-\y^k_1  \|^2,\notag
\end{eqnarray}
where $\uu_1$ is an arbitrary variable; in the inequality $\overset{a}\leq$,  we use the property that $f_1(\cdot)$ is convex, and so $f_1(\y^k_1)\leq f_1(\uu_1)+ \langle \nabla f_1(\y^k_1), \y^{k}-\uu\rangle $ and the inequality $\overset{b}\leq$ uses Eq.~\eqref{first}.   Then for $h_1(\cdot)$ is convex, and so $h_1(\x^{k+1}_1)\leq h_1(\uu_1)+ \langle \partial h_1(\x^{k+1}_1), \x^{k+1}-\uu_1\rangle$, we have 
\begin{eqnarray}
F_1(\x^{k+1}_1)&\leq& F_1(\uu_1) -\langle\A_1^T\blam(\y^k_1,\y^k_2)  ,\x^{k+1}_1-\uu_1 \rangle+\frac{L_1}{2}\| \x^{k+1}_1-\y^k_1  \|^2\notag\\
&&  -\left(L_1+\frac{\beta \| \A_1^T \A_1\|}{\theta_1}\right) \langle  \x^{k+1}_1-\y^{k}_1, \x^{k+1}_1-\uu_1\rangle.
\end{eqnarray}
Setting $\uu_1$  be $\x_1^{k}$, $\tx_1$ and $\x_1^*$, respectively, then multiplying the three inequalities by $(1-\theta_1-\theta_2)$, $\theta_2$, and $\theta_1$, respectively,  and adding them,  we have
\begin{eqnarray}\label{FF1}
&&F_1(\x^{k+1}_1)\\
&\leq& (1-\theta_1-\theta_2)F_1(\x^k_1)+ \theta_2 F_1(\tx_1)+\theta_1 F_1(\x_1^*)\notag\\
&&-\langle \A_1^T\blam(\y^k_1,\y^k_2)  ,\x^{k+1}_1-(1-\theta_1-\theta_2)\x^k_1-\theta_2\tx -\theta_1\x_1^*  \rangle \notag\\
&&  -\left(L_1+\frac{\beta \| \A_1^T \A_1\|}{\theta_1}\right) \langle  \x^{k+1}_1-\y^{k}_1, \x^{k+1}_1-(1-\theta_1-\theta_2)\x^k_1-\theta_2 \tx_1-\theta_1\x_1^*\rangle+\frac{L_1}{2}\|\x^{k+1}_1-\y^k_1  \|^2\notag\\
&\overset{a}\leq& (1-\theta_1-\theta_2)F_1(\x^k_1)+ \theta_2 F_1(\tx_1)+\theta_1 F_1(\x_1^*)\notag\\
&&-\langle \A_1^T\blam(\x^{k+1}_1,\y^k_2)  ,\x^{k+1}_1-(1-\theta_1-\theta_2)\x^k_1-\theta_2 \tx_1-\theta_1\x_1^*  \rangle \notag\\
&&  - \left\langle  \x^{k+1}_1-\y^{k}_1, \x^{k+1}_1-(1-\theta_1-\theta_2)\x^k_1-\theta_2\tx_1-\theta_1\x^*\right\rangle_{\left(L_1+\frac{\beta \| \A_1^T \A_1\|}{\theta_1}\right)\I-\frac{\beta\A_1^T\A_1}{\theta_1} }+\frac{L_1}{2}\|\x^{k+1}_1-\y^k_1  \|^2,\notag
\end{eqnarray}
where in the equality $\overset{a}\leq$, we replace $\A_1^T\blam(\y^k_1,\y^k_2)$ to be $\A_1^T\blam(\x^{k+1}_1,\y^k_2)-\frac{\beta\A^T_1\A_1}{\theta_1}(\x^{k+1}_1-\y^k_1)$.
For the optimal solution of $\x_2$, we have
\begin{eqnarray}\label{gradient}
\left(\alpha L_2+\frac{\beta \| \A_2^T \A_2\|}{\theta_1} \right) \left(\x^{k+1}_2-\y^{k}_2\right) + \tna f_2(\y^k_2) +\A_2^T\blam(\x^{k+1}_1,\y^k_2) \in -\partial h_2(\x^{k+1}_2),
\end{eqnarray} 
where we set $\alpha = 1+\frac{1}{b\theta_2}$. \\\\
\bfseries  Proof of step 2: \mdseries \\
Since $f_2$ have Lipschitz continuous gradients, we have
\begin{eqnarray}\label{f2}
f_2(\x^{k+1}_2)&\leq& f_2(\y^k_2) + \langle \nabla f_2(\y^k_2), \x^{k+1}_2 -\y^k_2 \rangle+\frac{L_2}{2}\|\x^{k+1}_2 -\y^k_2 \|^2.
\end{eqnarray}
We first consider $\langle  \nabla f_2(\y^k_2), \x^{k+1}_2 -\y^k_2 \rangle$. 
\begin{eqnarray}\label{adm1}
&&\langle \nabla f_2(\y^k_2), \x^{k+1}_2-\y^k_2  \rangle\notag\\
&\overset{a}=&\langle \nabla f_2(\y^k_2), \uu_2-\y^k_2+\x^{k+1}_2-\uu_2  \rangle \notag\\
&\overset{b}=& \langle \nabla f_2(\y^k_2),\uu_2-\y^k_2\rangle -\theta_3\langle \nabla f_2(\y^k_2), \y^k_2-\tx_2^s  \rangle +\langle \nabla f_2(\y^k_2),\z^{k+1}-\uu_2\rangle\notag\\
&=& \langle \nabla f_2(\y^k_2),\uu_2-\y^k_2\rangle -\theta_3\langle \nabla f_2(\y^k_2), \y^k_2-\tx_2^s  \rangle \notag\\
&& + \langle \tna f_2(\y^k_2),\z^{k+1}-\uu_2\rangle+ \langle \nabla f_2(\y^k_2)-\tna f_2(\y^k_2),\z^{k+1}-\uu_2\rangle,
\end{eqnarray}
where in the equality $\overset{a}=$, we introduce  an arbitrary variable $\uu_2$ (we will set it to be $\x_2^{k}$, $\tx_2$, and $\x_2^*$), and  in the equality $\overset{b}=$, we set $\z^{k+1} = \x^{k+1}_2 +\theta_3 (  \y^k_2 - \tx_2  ) $.
For $ \langle \tna f_2(\y_2^k),\z^{k+1}-\uu_2\rangle$, we have
\begin{eqnarray}\label{adm2}
&& \langle \tna f_2(\y_2^k),\z^{k+1}-\uu_2 \rangle\\
&\overset{a}=&  -\left\langle \partial h_2(\x^{k+1}_2) + \A_2^T\blam(\x^{k+1}_1,\y^k_2)+  \left(\alpha L_2+\frac{\beta \| \A_2^T \A_2\| }{\theta_1} \right)\left(\x^{k+1}_2-\y^{k}_2\right) ,  \z^{k+1}-\uu_2 \right\rangle \notag\\
&\overset{b}=& - \langle \partial h_2(\x^{k+1}_2), \x_2^{k+1}+\theta_{3}(\y^k_2-\tx_2)-\uu_2\rangle  \notag\\
&& - \left\langle  \A_2^T\blam(\x^{k+1}_1,\y^k_2)+  \left(\alpha L_2+\frac{\beta \| \A_2^T \A_2\|}{\theta_1} \right)\left(\x^{k+1}_2-\y^{k}_2\right) ,  \z^{k+1}-\uu_2 \right  \rangle \notag\\
&=& - \langle \partial h_2(\x^{k+1}_2), \x^{k+1}_2+\theta_3(\y^{k}_2 - \x_2^{k+1} + \x^{k+1}_2-\tx_2)-\uu_2\rangle  \notag\\
&& - \left\langle  \A_2^T\blam(\x^{k+1}_1,\y^k_2)+  \left(\alpha L_2+\frac{\beta \| \A_2^T \A_2\|}{\theta_1} \right)\left(\x^{k+1}_2-\y^{k}_2\right) ,  \z^{k+1}-\uu_2 \right  \rangle \notag\\
&\overset{c}\leq& h_2(\uu_2)-h_2(\x_2^{k+1}) + \theta_3h_2(\tx_2)-\theta_3h_2(\x_2^{k+1})- \theta_3\langle \partial h_2(\x^{k+1}_2), \y^k_2-\x^{k+1}_2 \rangle\notag\\
&&- \left\langle  \A_2^T\blam(\x^{k+1}_1,\y^k_2)+  \left(\alpha L_2+\frac{\beta \| \A_2^T \A_2\|}{\theta_1} \right)\left(\x^{k+1}_2-\y^{k}_2\right) ,  \z^{k+1}-\uu_2 \right  \rangle\notag\\
&\overset{d}=& h_2(\uu_2)-h_2(\x_2^{k+1}) + \theta_3h_2(\tx_2)-\theta_3h_2(\x_2^{k+1})\notag\\
&&- \left\langle  \A_2^T\blam(\x^{k+1}_1,\y^k_2)+  \left(\alpha L_2+\frac{\beta \| \A_2^T \A_2\|}{\theta_1} \right)\left(\x^{k+1}_2-\y^{k}_2\right) ,  \z^{k+1}-\uu_2 \right  \rangle\notag\\
&&-\theta_3\left\langle \A_2^T \blam(\x^{k+1}_1, \y^k_2)+            \left(\alpha L_2+\frac{\beta \| \A_2^T \A_2\|}{\theta_1} \right)\left(\x_2^{k+1}-\y_2^k\right)+\tna f_2(\y_2^k) ,\x_2^{k+1}-\y_2^k\right\rangle,\notag
\end{eqnarray}
where in the equalities $\overset{a}=$ and $\overset{d}=$,  we use Eq.~\eqref{gradient}; the inequality $\overset{b}=$ uses $\z^{k+1} = \x^{k+1}_2 +\theta_3 (  \y^k_2 - \tx_2  ) $; the inequality $\overset{c}\leq$ uses the  properties that:
$$\langle\partial h_2(\x^{k+1}_2), \uu_2-\x^{k+1}_2\rangle \leq h_2(\uu_2)-h_2(\x_2^{k+1}), $$ 
and 
$$\langle\partial h_2(\x^{k+1}_2), \tx_2-\x^{k+1}_2\rangle \leq h_2(\tx_2)-h_2(\x_2^{k+1}), $$
since $h_2(\cdot)$ is convex.  Adding Eq.~\eqref{adm1} and Eq.~\eqref{adm2}, and using $\tna f_2(\y_2^k)  =\nabla f_2(\y_2^k) +\tna f_2(\y_2^k)- \nabla f_2(\y_2^k)$, we obtain
\begin{eqnarray}\label{imm}
&&(1+\theta_3) \langle \nabla f_2(\y^k_2), \x^{k+1}_2-\y^k_2  \rangle\notag\\
&\leq& \langle \nabla f_2(\y^k_2),\uu_2-\y^k_2\rangle -\theta_3\langle \nabla f_2(\y^k_2), \y^k_2-\tx_2^s  \rangle+h_2(\uu_2)-h_2(\x_2^{k+1}) + \theta_3h_2(\tx_2)-\theta_3h_2(\x_2^{k+1})\notag\\
&&- \left\langle  \A_2^T\blam(\x^{k+1}_1,\y^k_2)+  \left(\alpha L_2+\frac{\beta \| \A_2^T \A_2\|}{\theta_1} \right)\left(\x^{k+1}_2-\y^{k}_2\right) ,  \z^{k+1}-\uu_2 +\theta_3( \x^{k+1}_2-\y^k_2) \right  \rangle\notag\\
&&+\langle \nabla f_2(\y^k_2)-\tna f_2(\y^k_2),\theta_3(\x^{k+1}_2-\y^k_2)+\z^{k+1}-\uu_2\rangle.
\end{eqnarray}
Multiplying Eq.~\eqref{f2} by $(1+\theta_3)$  and then adding Eq.~\eqref{imm},  we can eliminate the term $\langle \nabla f_2(\y^k_2), \x^{k+1}_2-\y^k_2  \rangle$ and  obtain
\begin{eqnarray}\label{noexpectation}
&&(1+\theta_3)F_2(\x^{k+1}_2)  \notag\\
&\leq& (1+\theta_3) f_2(\y^k_2)+\langle\nabla f_2(\y^k_2), \uu_2-\y^k_2\rangle -\theta_3\langle\nabla f_2(\y^k_2), \y^k_2 -\tx_2\rangle + h_2(\uu_2)+\theta_3 h_2(\tx_2)\notag\\
&&- \left\langle  \A_2^T\blam(\x^{k+1}_1,\y^k_2)+  \left(\alpha L_2+\frac{\beta \| \A_2^T \A_2\|}{\theta_1} \right)\left(\x^{k+1}_2-\y^{k}_2\right) ,  \z^{k+1}-\uu_2 +\theta_3( \x^{k+1}_2-\y^k_2) \right  \rangle\notag\\
&&+\langle \nabla f_2(\y^k_2)-\tna f_2(\y^k_2),\theta_3(\x^{k+1}_2-\y^k_2)+\z^{k+1}-\uu_2\rangle+\frac{(1+\theta_3)L_2}{2}\| \x^{k+1}_2-\y_2^k\|^2\notag\\
&\overset{a}\leq& F_2(\uu_2)-\theta_3\langle\nabla f(\y^k_2), \y^k_2 -\tx_2\rangle +\theta_3 f_2(\y^k_2) + \theta_3 h_2(\tx_2)\notag\\
&&- \left\langle  \A_2^T\blam(\x^{k+1}_1,\y^k_2)+  \left(\alpha L_2+\frac{\beta \| \A_2^T \A_2\|}{\theta_1} \right)\left(\x^{k+1}_2-\y^{k}_2\right) ,  \z^{k+1}-\uu_2 +\theta_3( \x^{k+1}_2-\y^k_2) \right  \rangle\notag\\
&&+\langle \nabla f(\y^k_2)-\tna f_2(\y^k_2),\theta_3(\x^{k+1}_2-\y^k_2)+\z^{k+1}-\uu_2\rangle+\frac{(1+\theta_3)L_2}{2}\| \x^{k+1}_2-\y_2^k\|^2,
\end{eqnarray}
where the inequality $\overset{a}\leq$ uses the property that $\langle\nabla f_2(\y^k_2), \uu_2-\y^k_2\rangle \leq f_2(\uu_2)-f_2(\y^k_2).$ 

We now consider the term $\langle \nabla f_2(\y^k_2)-\tna f_2(\y^k_2),\theta_3(\x^{k+1}_2-\y^k_2)+\z^{k+1}-\uu_2\rangle$. We will set $\uu_2$ be $\x_2^k$ and $\x^*_2$, they do not depend on $i_{k,s}$. So we obtain
\begin{eqnarray}\label{variance1}
&&\E_{i_{k}}\left(\left\langle \nabla f_2(\y_2^k) - \tna f_2(\y^k), \theta_3(\x_2^{k+1}-\y_2^k)+\z^{k+1}-\uu_2  \right\rangle\right) \notag\\
&=& \E_{i_{k}}\left(\left\langle \nabla f_2(\y_2^k) - \tna f_2(\y_2^k), \theta_3\z^{k+1}+ \z^{k+1}\right\rangle\right) -  \E_{i_{k}}\left(\left\langle \nabla f_2(\y_2^k) - \tna f_2(\y_2^k), \theta^2_3(\y_2^k-\tx_2)+\theta_3\y_2^k+\uu_2 \right\rangle\right) \notag\\
&\overset{a}=& (1+\theta_3)\E_{i_{k}}(\langle \nabla f_2(\y_2^k) - \tna f_2(\y_2^k), \z^{k+1}\rangle) \notag\\
&\overset{b}=& (1+\theta_3)\E_{i_{k}}(\langle \nabla f_2(\y_2^k) - \tna f_2(\y_2^k), \x_2^{k+1}\rangle) \notag\\
&\overset{c}=& (1+\theta_3)\E_{i_{k}}(\langle \nabla f_2(\y^k_2) - \tna f_2(\y^k_2), \x_2^{k+1}-\y_2^{k}\rangle) \notag\\
&\overset{d}\leq& \E\left( \frac{\theta_3b}{2 L_2}\|\nabla f_2(\y^k_2) - \tna f_2(\y^k_2)\|^2   \right)+  \E\left( \frac{(1+\theta_3)^2 L_2}{2\theta_3 b}\| \x_2^{k+1}-\y_2^{k}\|^2 \right),
\end{eqnarray}
where in the equality $\overset{a}=$, we use the fact that
$$\E_{i_k} \left(\nabla f_2(\y^k_2) - \tna f_2(\y^k_2) \right)=\mathbf{0},$$
and $\x^k_2$, $\uu_2$, and $\tx_2$ are independent of $i_{k,s}$ (are known), so 
\begin{eqnarray}
\E_{i_k} \langle \nabla f_2(\y^k_2) - \tna f_2(\y^k_2), \x^k_2 \rangle =0,\notag\\
\E_{i_k} \langle \nabla f_2(\y^k_2) - \tna f_2(\y^k_2),\y^k_2 \rangle =0,\notag\\
\E_{i_k} \langle \nabla f_2(\y^k_2) - \tna f_2(\y^k_2), \uu^k_2 \rangle =0;\notag
\end{eqnarray}
the inequalities $\overset{b}\leq$ and  $\overset{c}\leq$ hold similarly; the equality $\overset{d}\leq$ uses the Cauchy-Schwarz inequality. Substituting Eq.~\eqref{boundd} into Eq.~\eqref{variance1}, and taking expectation on Eq.~\eqref{noexpectation}, and add them, we obtain
\begin{eqnarray}
&&(1+\theta_3)\E_{i_{k}}\left(F_2(\x^{k+1}_2) \right) \notag\\
&\overset{a}\leq&- \E_{i_{k}}\left\langle  \A_2^T\blam(\x^{k+1}_1,\y^k_2)+  \left(\alpha L_2+\frac{\beta\| \A_2^T \A_2\|}{\theta_1} \right)\left(\x^{k+1}_2-\y^{k}_2\right) ,  \z^{k+1}-\uu_2 +\theta_3( \x^{k+1}_2-\y^k_2) \right  \rangle\notag\\
&&+ F_2(\uu_2) +\theta_3 F(\tx_2) +\E_{i_{k}}\left( \frac{(1+\theta_3)(1+\frac{1}{b\theta_2})L_2}{2}\| \x^{k+1}_2-\y^k_2\|^2 \right)\notag\\
&\overset{b}=&- \E_{i_{k}}\left\langle  \A_2^T\blam(\x^{k+1}_1,\y^k_2)+  \left(\alpha L_2+\frac{\beta\| \A_2^T \A_2\|}{\theta_1} \right)\left(\x^{k+1}_2-\y^{k}_2\right) ,  (1+\theta_3)\x^{k+1}_2 -\theta_3\tx_2-\uu_2  \right  \rangle\notag\\
&&+ F_2(\uu_2) +\theta_3 F(\tx_2) +\E_{i_{k}}\left( \frac{(1+\theta_3)(1+\frac{1}{b\theta_2})L_2}{2}\| \x^{k+1}_2-\y^k_2\|^2 \right),
\end{eqnarray}
where in the equality $\overset{a}\leq$, we set $\theta_2 = \frac{\theta_3}{1+\theta_3}$;  inequality $\overset{b}\leq$ uses $\z^{k+1} = \x^{k+1}_2 +\theta_3 (  \y^k_2 - \tx_2  ) $. Setting $\uu_2$  be $\x_2^{k}$  and $\x_2^*$, respectively, then multiplying  the two inequalities by $1-\theta_1(1+\theta_3)$ and $\theta_1(1+\theta_3)$, and adding them, we obtain
\begin{eqnarray}\label{bff2}
&&(1+\theta_3)\E_{i_{k}}\left(F_2(\x^{k+1}_2) \right)\notag\\
&\leq&- \E_{i_{k}}\left\langle  \A_2^T\blam(\x^{k+1}_1,\y^k_2)+  \left(\alpha L_2+\frac{\beta\| \A_2^T \A_2\|}{\theta_1} \right)\left(\x^{k+1}_2-\y^{k}_2\right) ,  (1+\theta_3)\x^{k+1}_2 -\theta_3\tx_2 \right  \rangle\notag\\
&&- \E_{i_{k}}\left\langle  \A_2^T\blam(\x^{k+1}_1,\y^k_2)+  \left(\alpha L_2+\frac{\beta\| \A_2^T \A_2\|}{\theta_1} \right)\left(\x^{k+1}_2-\y^{k}_2\right) ,  -\left(1-\theta_1(1+\theta_3) \right)\x_2^{k} \right  \rangle\notag\\
&&- \E_{i_{k}}\left\langle  \A_2^T\blam(\x^{k+1}_1,\y^k_2)+  \left(\alpha L_2+\frac{\beta\| \A_2^T \A_2\|}{\theta_1} \right)\left(\x^{k+1}_2-\y^{k}_2\right) ,  -\left(\theta_1(1+\theta_3)\right)\x_2^* \right  \rangle\notag\\
&&+ \left(1-\theta_1(1+\theta_3)\right)F_2(\x_2^k) +\left(\theta_1(1+\theta_3)\right) F_2(\x_2^*) +\theta_3 F(\tx_2)\notag\\
&& +\E_{i_{k}}\left( \frac{(1+\theta_3)(1+\frac{1}{b\theta_2})L_2}{2}\| \x^{k+1}_2-\y^k_2\|^2 \right).
\end{eqnarray}
Dividing Eq.~\eqref{bff2} by $(1+\theta_3)$, we obtain
\begin{eqnarray}\label{FF2}
&&\E_{i_{k}}F_2(\x^{k+1}_2)\notag\\
&\leq&- \E_{i_{k}}\left\langle  \A_2^T\blam(\x^{k+1}_1,\y^k_2)+  \left(\alpha L_2+\frac{\beta\| \A_2^T \A_2\|}{\theta_1} \right)\left(\x^{k+1}_2-\y^{k}_2\right) ,  \x^{k+1}_2 -\theta_2\tx_2\right  \rangle\notag\\
&&- \E_{i_{k}}\left\langle  \A_2^T\blam(\x^{k+1}_1,\y^k_2)+  \left(\alpha L_2+\frac{\beta\| \A_2^T \A_2\|}{\theta_1} \right)\left(\x^{k+1}_2-\y^{k}_2\right) ,  - (1-\theta_2-\theta_1)\x^k_{2}-\theta_1\x_2^* \right  \rangle\notag\\
&&+(1-\theta_2-\theta_1)F_2(\x^{k}_2) +\theta_1F_2(\x_2^*) +\theta_2 F_2(\tx_2) +\E_{i_{k}}\left( \frac{(1+\frac{1}{b\theta_2})L_2}{2}\| \x^{k+1}_2-\y^k_2\|^2 \right),
\end{eqnarray}
where we use $\theta_2=\frac{\theta_3}{1+\theta_3}$ and so $\frac{1-\theta_1(1+\theta_3)}{1+\theta_3}=1-\theta_2-\theta_1$.\\\\
\bfseries  Proof of step 3: \mdseries \\
Setting $\hlam^{k} = \tlam^{k} +\frac{\beta(1-\theta_1)}{\theta_1}(\A_1\x^{k}_1+\A_2\x^{k}_2-\b)$, we have
\begin{eqnarray}\label{hlamlist}
&&\hlam^{k+1}\\
&=&\tlam^{k+1}  +\beta \left(\frac{1}{\theta_1}-1\right)(\A_1\x^{k+1}_1+\A_2\x^{k+1}_2-\b)\notag\\
&\overset{a}=&\olam^{k}  +\frac{\beta }{\theta_1}(\A_1\x^{k+1}_1+\A_2\x^{k+1}_2-\b)\notag\\
&\overset{b}=&\blam(\x^{k+1}_1,\x^{k+1}_2)\notag\\
&\overset{c}=& \tlam^k +\frac{\beta}{\theta_1}\left( \A_1\x^{k+1}_1+\A_2\x^{k+1}_2-\b +\theta_2\left( \A_1(\x^{k}_2-\tx_1) + \A_2(\x^{k}_2-\tx_2)\right) \right),\notag
\end{eqnarray}
where in equality $\overset{a}=$, we use Eq.~(11) in the paper;  the equality $\overset{c}=$ is obtained through Eq.~(10) in the paper. Using  $\hlam^{k} = \tlam^{k} +\frac{\beta(1-\theta_1)}{\theta_1}(\A_1\x^{k}_1+\A_2\x^{k}_2-\b)$, we obtain
\begin{eqnarray}\label{nolis1}
&&\hlam^{k+1}-\hlam^{k} \notag\\
&=& \frac{\beta A_1}{\theta_1}\left(\x^{k+1}_1-(1-\theta_1)\x_1^{k}-\theta_1\x_1^* +\theta_2(\x^k_1-\tx_1)\right)\notag\\
&&+ \frac{\beta A_2}{\theta_1}\left(\x^{k+1}_2-(1-\theta_1)\x_2^{k}-\theta_1\x_2^* +\theta_2(\x^k_2-\tx_2) \right),
\end{eqnarray}
where we use the fact that $\A_1\x_1^*+\A_2\x_2^*=\b$. Now we prove $\hlam^m_{s-1} =  \hlam^0_{s}$ when $s\geq 1$.
\begin{eqnarray}\label{lams1}
&&\hlam^0_{s}\notag\\
&=&\tlam^0_s+ \frac{\beta(1-\theta_{1,s})}{\theta_{1,s}}\left( \A_1\x^m_{s,1} +\A_2\x^{m}_{s,2}-\b\right)\notag\\
&\overset{a}=&\tlam^0_s+ \beta \left(\frac{1}{\theta_{1,{s-1}}}+\tau-1\right)\left( \A_1\x^m_{s,1} +\A_2\x^{m}_{s,2}-\b\right)\notag\\
&\overset{b}=&\olam^{m-1}_{s-1} -\beta (\tau-1) \left( \A_1\x^m_{s,1} +\A_2\x^{m}_{s,2}-\b\right)+\beta (\frac{1}{\theta_{1,s-1}}+\tau-1) \left( \A_1\x^m_{s,1} +\A_2\x^{m}_{s,2}-\b\right)\notag\\
&=&\olam^{m-1}_{s-1} +\frac{\beta}{\theta_{1,s-1}} \left( \A_1\x^m_{s,1} +\A_2\x^{m}_{s,2}-\b\right)\notag\\
&\overset{c}=&\tlam^{m}_{s-1} -(\beta-\frac{\beta}{\theta_{1,s-1}})\left( \A_1\x^m_{s,1} +\A_2\x^{m}_{s,2}-\b\right) =\hlam^m_{s-1},
\end{eqnarray}
where the equality $\overset{a}=$ uses the fact that  $\frac{1}{\theta_{1,s}}=\frac{1}{\theta_{1,s-1}}+\tau$;  the equality $\overset{b}=$  uses Eq.~(12) in the paper;  the equality $\overset{c}=$  uses Eq.~(11) in the paper.\\\\\\\\\\
\bfseries  Proof of Lemma 1: \mdseries \\

Define $L(\x_1,\x_2,\olam) =  F_1(\x_1) - F_1(\x^*_1)+ F_2(\x_2)-F_2(\x^*_2) + \langle \olam, \A_1\x_1+\A_2\x_2-\b  \rangle$. We have
\begin{eqnarray}
&&L(\x^{k+1}_1,\x^{k+1}_2,\olam^*) - \theta_2 L(\tx_1,\tx_2,\olam^*) -(1-\theta_1 - \theta_2)L(\x^{k}_1,\x^{k}_2,\olam^*)\notag\\ 
&=& F_1(\x^{k+1}_1)-(1-\theta_2-\theta_1)F_1(\x^{k}_1) -\theta_1F_1(\x^*_1) -\theta_2 F_1(\tx_1)\notag\\
&&+F_2(\x^{k+1}_2)-(1-\theta_2-\theta_1)F_2(\x^{k}_2) -\theta_1F_2(\x^*_2) -\theta_2 F_2(\tx_2)\notag\\
&&+ \left\langle \olam^*, \A_1\left[\x^{k+1}_1-(1-\theta_1-\theta_2)\x_1^{k}-\theta_2\tx_1-\theta_1 \x_1^*\right]   \right)\rangle\notag\\
&&+ \left\langle \olam^*, \A_2\left[\x^{k+1}_2-(1-\theta_1-\theta_2)\x_2^{k}-\theta_2\tx_2-\theta_1 \x_2^*\right]  \right)\rangle.
\end{eqnarray}
Adding Eq.~\eqref{FF1} and Eq.~\eqref{FF2}, we have 
\begin{eqnarray}\label{nolis}
&& \E_{i_k}\left(L(\x^{k+1}_1,\x^{k+1}_2,\olam^*)\right) - \theta_2 L(\tx_1,\tx_2,\olam^*) -(1-\theta_2 - \theta_1)L(\x^{k}_1,\x^{k}_2,\olam^*)\notag\\ 
&\leq& \E_{i_k}\left\langle \olam^*-\blam(\x^{k+1}_1,\y^k_2),   \A_1\left[\x^{k+1}_1-(1-\theta_1-\theta_2)\x_1^{k}-\theta_2\tx_1-\theta_1 \x_1^*\right]   \right\rangle\notag\\
&&+\E_{i_k}\left\langle \olam^*-\blam(\x^{k+1}_1,\y^k_2),  \A_2\left[\x^{k+1}_2-(1-\theta_1-\theta_2)\x_2^{k}-\theta_2\tx_2-\theta_1 \x_2^*\right]  \right\rangle\notag\\
&&  - \E_{i_k}\left\langle  \x^{k+1}_1-\y^{k}_1, \x^{k+1}_1-(1-\theta_1-\theta_2)\x_1^{k}-\theta_2\tx_1-\theta_1 \x_1^*\right\rangle_{\left(L_1+\frac{\beta\| \A_1^T \A_1\|}{\theta_1}\right)\I-\frac{\beta\A_1^T\A_1}{\theta_1} }\notag\\
&& -\E_{i_k}\left\langle\x^{k+1}_2-\y^{k}_2 ,  \x^{k+1}_2 -\theta_2\tx_2- (1-\theta_2-\theta_1)\x^k_{2}-\theta_1\x^* \right  \rangle_{\left(\alpha L_2+\frac{\beta\| \A_2^T \A_2\|}{\theta_1}\right)\I}\notag\\
&&+\frac{L_1}{2}\E_{i_k}\|\x^{k+1}_1-\y^k_1  \|^2+\E_{i_k}\left( \frac{(1+\frac{1}{b\theta_2})L_2}{2}\| \x^{k+1}_2-\y^k_2\|^2 \right)\notag\\
&\overset{a}=&\E_{i_k}\left\langle \olam^*-\blam(\x^{k+1}_1,\x^{k+1}_2),   \A_1\left[\x^{k+1}_1-(1-\theta_1-\theta_2)\x_1^{k}-\theta_2\tx_1-\theta_1 \x_1^*\right]   \right\rangle\notag\\
&&+\E_{i_k}\left\langle \olam^*-\blam(\x^{k+1}_1,\x^{k+1}_2),  \A_2\left[\x^{k+1}_2-(1-\theta_1-\theta_3)\x_2^{k}-\theta_2\tx_2-\theta_1 \x_2^*\right]  \right\rangle\notag\\
&&  - \E_{i_k}\left\langle  \x^{k+1}_1-\y^{k}_1,\x^{k+1}_1-(1-\theta_1-\theta_2)\x_1^{k}-\theta_2\tx_1-\theta_1 \x_1^*\right\rangle_{\left(L_1+\frac{\beta \| \A_1^T \A_1\|}{\theta_1}\right)\I-\frac{\beta\A_1^T\A_1}{\theta_1} }\notag\\
&& -\E_{i_k}\left\langle\x^{k+1}_2-\y^{k}_2 ,  \x^{k+1}_2 -\theta_2\tx_2- (1-\theta_2-\theta_1)\x^k_{2}-\theta_1\x^* \right  \rangle_{\left(\alpha L_2+\frac{\beta \| \A_2^T \A_2\|}{\theta_1}\right)\I-\frac{\beta\A^T_2\A_2}{\theta_1}}\notag\\
&&+\frac{L_1}{2}\E_{i_k}\|\x^{k+1}_1-\y^k_1  \|^2+\E_{i_k}\left( \frac{(1+\frac{1}{b\theta_2})L_2}{2}\| \x^{k+1}_2-\y^k_2\|^2 \right)\notag\\
&&+\frac{\beta}{\theta_1}\E_{i_k}\left\langle \A_2\x^{k+1}_2-\A_2\y^{k}_2,\A_1\left[\x^{k+1}_1-(1-\theta_1-\theta_2)\x_1^{k}-\theta_2\tx_1-\theta_1 \x_1^*\right]   \right\rangle,
\end{eqnarray}
where in the equality $\overset{a}=$, we change the term $\blam(\x^{k+1}_1,\y_2^k)$ to $\blam(\x^{k+1}_1,\x_2^{k+1})-\frac{\beta\A^T_2\A_2}{\theta_1}(\x^{k+1}_2-\y^k_2)$. 
Now we analyse Eq.~\eqref{nolis}. For the first two terms in the right hand of Eq.~\eqref{nolis}, we have
\begin{eqnarray}\label{llam}
&&\left\langle \olam^*-\blam(\x^{k+1}_1,\x^{k+1}_2),   \A_1\left[\x^{k+1}_1-(1-\theta_1-\theta_2)\x_1^{k}-\theta_2\tx_1-\theta_1\x_1^*\right]   \right\rangle\notag\\
&&+\left\langle \olam^*-\blam(\x^{k+1}_1,\x^{k+1}_2),  \A_2\left[\x^{k+1}_2-(1-\theta_1-\theta_2)\x_1^{k}-\theta_2\tx_2-\theta_1 \x_2^*\right]  \right\rangle\notag\\
&=& \frac{\theta_1}{\beta} \langle \olam^*-\hlam^{k+1}, \hlam^{k+1}-\hlam^{k}\rangle\notag\\
&=& \frac{\theta_1}{2\beta}\left(\|\hlam^k-\olam^*\|^2- \|\hlam^{k+1}-\olam^*\|^2 -\| \hlam^{k+1} -\hlam^{k}\|^2\right).
\end{eqnarray}
where in the first equality, we use $\overset{b}=$ in Eq.~\eqref{hlamlist} and Eq.~\eqref{nolis1}, and in the second equality we use the fact that 
$$\langle \mathbf{a}-\b, \mathbf{a}-\mathbf{c}\rangle = \frac{1}{2}\|\mathbf{a}-\b\|^2+\frac{1}{2}\|\mathbf{a}-\mathbf{c}\|^2-\frac{1}{2}\|\mathbf{b}-\mathbf{c}\|^2.  $$
For the last term in the right hand of Eq.~\eqref{nolis}, we have
\begin{eqnarray}\label{nolis2}
&&\frac{\beta}{\theta_1}\left\langle \A_2\x^{k+1}_2-\A_2\y^{k}_2,\A_1\left[\x^{k+1}_1-(1-\theta_1-\theta_2)\x_1^{k}-\theta_2\tx_1-\theta_1\x_1^*\right]   \right\rangle\notag\\
&\overset{a}=&\frac{\beta}{\theta_1}\left\langle \A_2\x^{k+1}_2-\A_2\vv -(\A_2\y^{k}_2-\A_2\vv),\A_1\left[\x^{k+1}_1-(1-\theta_1-\theta_2)\x_1^{k}-\theta_2\tx_1-\theta_1\x_1^*\right] -\mathbf{0}  \right\rangle\notag\\
&\overset{b}=&\frac{\beta}{2\theta_1}\|\A_2\x^{k+1}_2 -\A_2 \vv+  \A_1\left[\x^{k+1}_1-(1-\theta_1-\theta_2)\x_1^{k}-\theta_2\tx_1-\theta_1\x_1^*\right]   \|^2-\frac{\beta}{2\theta_1}\| \A_2\x^{k+1}_2-\A_2\vv  \|^2\notag\\
&&+\frac{\beta}{2\theta_1}\|  \A_2\y^{k}_2-\A_2\vv \|^2-\frac{\beta}{2\theta_1}\|\A_2\y^{k}_2-\A_2 \vv +  \A_1\left(\x^{k+1}_1-(1-\theta_1-\theta_2)\x_1^{k}-\theta_2\tx_1-\theta_1\x_1^*\right)   \|^2,\notag\\
&\overset{c}=& \frac{\theta_1}{2\beta}\| \hlam^{k+1} -\hlam^{k}  \|^2 -\frac{\beta}{2\theta_1}\| \A_2\x^{k+1}_2-\A_2\vv  \|^2+\frac{\beta}{2\theta_1}\|  \A_2\y^{k}_2-\A_2\vv \|^2\notag\\
&&-\frac{\beta}{2\theta_1}\|\A_2\y^{k}_2-\A_2 \vv +  \A_1\left(\x^{k+1}_1-(1-\theta_1-\theta_2)\x_1^{k}-\theta_2\tx_1-\theta_1\x_1^*\right)   \|^2,
\end{eqnarray}
where in the  equality $\overset{a}=$, we set $\vv=(1-\theta_1-\theta_2)\x_2^{k}+\theta_2\tx_2+\theta_1 \x_2^*$;  the equality $\overset{b}=$ uses the fact that 
$$\langle \mathbf{a}- \mathbf{b}, \mathbf{c}- \mathbf{d} \rangle = \frac{1}{2}\left(\| \mathbf{a}+ \mathbf{c}\|^2-\| \mathbf{a}+ \mathbf{d}\|^2+\| \mathbf{b}+ \mathbf{d}\|^2-\| \mathbf{b}+ \mathbf{c}\|^2 \right),$$
and the equality $\overset{c}=$ uses Eq.~\eqref{hlamlist}.  For the third and fourth terms in the right hand of Eq.~\eqref{nolis}, we have
\begin{eqnarray}\label{nolis3}
&&\langle \x_i^{k+1}-\y_i^k, \x_i^{k+1}-(1-\theta_1-\theta_2)\x_i^k-\theta_2\tx_i-\theta_1\x_i^*\rangle_{\G_i}\notag\\
&\leq& \frac{1}{2}\left(\|\x_i^{k+1}-(1-\theta_1-\theta_2)\x_i^k-\theta_2\tx_i-\theta_1\x_i^* \|^2_{\G_i} -  \| \x_i^{k+1}-\y_i^k \|^2_{\G_i}\right)\notag\\
&&- \|\y_i^{k}-(1-\theta_1-\theta_2)\x_i^k-\theta_2\tx_i-\theta_1\x_i^*\|^2_{\G_i} ,\quad i=1,2,
\end{eqnarray}
where $\G_1 = \left(L_1+\frac{\beta \| \A_1^T \A_1\|}{\theta_1}\right)\I-\frac{\beta\A_1^T\A_1}{\theta_1} $  and $\G_2=\left(\alpha L_2+\frac{\beta\| \A_2^T \A_2\|}{\theta_1}\right)\I-\frac{ \beta\A_2^T \A_2}{\theta_1}$.
So substituting Eq~\eqref{llam} into Eq.~\eqref{nolis}, we obtain:
\begin{eqnarray}\label{temm}
&& \E_{i_k}\left(L(\x^{k+1}_1,\x^{k+1}_2,\olam^*)\right) - \theta_2 L(\tx_1,\tx_2,\olam^*) -(1-\theta_2 - \theta_1)L(\x^{k}_1,\x^{k}_2,\olam^*)\notag\\ 
&\leq& \frac{\theta_1}{2\beta}\left(\|\hlam^k-\olam^*\|^2- \|\hlam^{k+1}-\olam^*\|^2 -\| \hlam^{k+1} -\hlam^{k}\|^2\right)\notag\\
&&  +\E_{i_k}\left\langle  \x^{k+1}_1-\y^{k}_1,\x^{k+1}_1-(1-\theta_1-\theta_2)\x_1^{k}-\theta_2\tx_1-\theta_1 \x_1^*\right\rangle_{\left(L_1+\frac{\beta \| \A_1^T \A_1\|}{\theta_1}\right)\I-\frac{\beta\A_1^T\A_1}{\theta_1} }\notag\\
&& -\E_{i_k}\left\langle\x^{k+1}_2-\y^{k}_2 ,  \x^{k+1}_2 -\theta_2\tx_2- (1-\theta_2-\theta_1)\x^k_{2}-\theta_1\x^* \right  \rangle_{\left(\alpha L_2+\frac{\beta \| \A_2^T \A_2\|}{\theta_1}\right)\I-\frac{\beta\A^T_2\A_2}{\theta_1}}\notag\\
&&+\frac{L_1}{2}\E_{i_k}\|\x^{k+1}_1-\y^k_1  \|^2+\E_{i_k}\left( \frac{(1+\frac{1}{b\theta_2})L_2}{2}\| \x^{k+1}_2-\y^k_2\|^2 \right)\notag\\
&&+\frac{\beta}{\theta_1}\E_{i_k}\left\langle \A_2\x^{k+1}_2-\A_2\y^{k}_2,\A_1\left[\x^{k+1}_1-(1-\theta_1-\theta_2)\x_1^{k}-\theta_2\tx_1-\theta_1 \x_1^*\right]   \right\rangle.
\end{eqnarray}
Then substituting Eq~\eqref{nolis3} into Eq.~\eqref{temm}, we obtain:
\begin{eqnarray}\label{temm2}
&& \!\!\!\!\!\!\!\E_{i_k}\left(L(\x^{k+1}_1,\x^{k+1}_2,\olam^*)\right) - \theta_2 L(\tx_1,\tx_2,\olam^*) -(1-\theta_2 - \theta_1)L(\x^{k}_1,\x^{k}_2,\olam^*)\\
&\leq&  \frac{\theta_1}{2\beta}\left(\|\hlam^k-\olam^*\|^2- \E_{i_k}\|\hlam^{k+1}-\olam^*\|^2 -\E_{i_k}\| \hlam^{k+1} -\hlam^{k}\|^2\right)\notag\\
&&+\frac{1}{2}\|\y_1^{k}-(1-\theta_1-\theta_2)\x_1^{k}-\theta_2\tx_1-\theta_1\x_1^*\|^2_{\left(L_1+\frac{\| \beta\A_1^T \A_1\|}{\theta_1}\right)\I-\frac{\beta\A_1^T\A_1}{\theta_1} }\notag\\
&&-\frac{1}{2}\E_{i_k}\left(\|\x^{k+1}_1-(1-\theta_1-\theta_2)\x_1^{k}-\theta_2\tx_1-\theta_1\x_1^*\|^2_{\left(L_1+\frac{\beta\| \A_1^T \A_1\|}{\theta_1}\right)\I-\frac{\beta\A_1^T\A_1}{\theta_1} }\right)\notag\\
&&+ \frac{1}{2} \|\y_2^{k}-(1-\theta_1-\theta_2)\x^k_2-\theta_2\tx_2-\theta_1\x_2^*\|^2_{\left(\alpha L_2+\frac{\beta\| \A_2^T \A_2\|}{\theta_1}\right)\I-\frac{\beta\A_2^T\A_2}{\theta_1}}\notag\\
&&-\frac{1}{2} \E_{i_k} \left(\|\x_2^{k+1}-(1-\theta_1-\theta_2)\x^k_2-\theta_2\tx_2-\theta_1\x_2^*\|^2_{\left(\alpha L_2+\frac{\beta\| \A_2^T \A_2\|}{\theta_1}\right)\I-\frac{\beta\A_2^T\A_2}{\theta_1}}\right)\notag\\
&&-\E_{i_k}\|\x^{k+1}_1-\y^k_1  \|^2_{\left(\frac{\beta\| \A_1^T \A_1\|}{\theta_1}\right)\I-\frac{\beta\A_1^T\A_1}{\theta_1} }-\E_{i_k}\| \x^{k+1}_2-\y^k_2\|^2_{\left(\frac{\beta\| \A_2^T \A_2\|}{\theta_1}\right)\I-\frac{\beta\A_2^T\A_2}{\theta_1} } \notag\\
&&+\frac{\beta}{\theta_1}\E_{i_k}\left\langle \A_2\x^{k+1}_2-\A_2\y^{k}_2,\A_1\left[\x^{k+1}_1-(1-\theta_1-\theta_2)\x_1^{k}-\theta_2\tx_1-\theta_1 \x_1^*\right]   \right\rangle.\notag
\end{eqnarray}
Substituting  Eq.~\eqref{nolis2} into Eq.~\eqref{temm2}, we have
\begin{eqnarray}\label{anns1}
&& \!\!\!\!\!\!\!\E_{i_k}\left(L(\x^{k+1}_1,\x^{k+1}_2,\olam^*)\right) - \theta_2 L(\tx_1,\tx_2,\olam^*) -(1-\theta_2 - \theta_1)L(\x^{k}_1,\x^{k}_2,\olam^*)\\
&\leq&  \frac{\theta_1}{2\beta}\left(\|\hlam^k-\olam^*\|^2- \E_{i_k}\|\hlam^{k+1}-\olam^*\|^2 \right)\notag\\
&&+\frac{1}{2}\|\y_1^{k}-(1-\theta_1-\theta_2)\x_1^{k}-\theta_2\tx_1-\theta_1\x_1^*\|^2_{\left(L_1+\frac{\beta\| \A_1^T \A_1\|}{\theta_1}\right)\I-\frac{\beta\A_1^T\A_1}{\theta_1} }\notag\\
&&-\frac{1}{2}\E_{i_k}\left(\|\x^{k+1}_1-(1-\theta_1-\theta_2)\x_1^{k}-\theta_2\tx_1-\theta_1\x_1^*\|^2_{\left(L_1+\frac{\beta\| \A_1^T \A_1\|}{\theta_1}\right)\I-\frac{\beta\A_1^T\A_1}{\theta_1} }\right)\notag\\
&&+ \frac{1}{2} \|\y_2^{k}-(1-\theta_1-\theta_2)\x^k_2-\theta_2\tx_2-\theta_1\x_2^*\|^2_{\left(\alpha L_2+\frac{\beta\| \A_2^T \A_2\|}{\theta_1}\right)\I}\notag\\
&&-\E_{i_k}\|\x^{k+1}_1-\y^k_1  \|^2_{\left(\frac{\beta\| \A_1^T \A_1\|}{\theta_1}\right)\I-\frac{\beta\A_1^T\A_1}{\theta_1} }-\E_{i_k}\| \x^{k+1}_2-\y^k_2\|^2_{\left(\frac{\beta\| \A_2^T \A_2\|}{\theta_1}\right)\I-\frac{\beta\A_2^T\A_2}{\theta_1} } \notag\\
&&-\frac{\beta}{2\theta_1}\E_{i_k}\|\A_2\y^{k}_2-\A_2 \vv +  \A_1\left(\x^{k+1}_1-(1-\theta_1-\theta_2)\x_1^{k}-\theta_2\tx_1-\theta_1\x_1^*\right)   \|^2.\notag
\end{eqnarray}
Since the last three terms in the right hand of  Eq.~\eqref{anns1} are nonpositive, we obtain:
\begin{eqnarray}
&& \!\!\!\!\!\!\!\E_{i_k}\left(L(\x^{k+1}_1,\x^{k+1}_2,\olam^*)\right) - \theta_2 L(\tx_1,\tx_2,\olam^*) -(1-\theta_2 - \theta_1)L(\x^{k}_1,\x^{k}_2,\olam^*)\\
&\leq&  \frac{\theta_1}{2\beta}\left(\|\hlam^k-\olam^*\|^2- \E_{i_k}\|\hlam^{k+1}-\olam^*\|^2 \right)\notag\\
&&+\frac{1}{2}\|\y_1^{k}-(1-\theta_1-\theta_2)\x_1^{k}-\theta_2\tx_1-\theta_1\x_1^*\|^2_{\left(L_1+\frac{\beta\| \A_1^T \A_1\|}{\theta_1}\right)\I-\frac{\beta\A_1^T\A_1}{\theta_1} }\notag\\
&&-\frac{1}{2}\E_{i_k}\left(\|\x^{k+1}_1-(1-\theta_1-\theta_2)\x_1^{k}-\theta_2\tx_1-\theta_1\x_1^*\|^2_{\left(L_1+\frac{\beta\| \A_1^T \A_1\|}{\theta_1}\right)\I-\frac{\beta\A_1^T\A_1}{\theta_1} }\right)\notag\\
&&+ \frac{1}{2} \|\y_2^{k}-(1-\theta_1-\theta_2)\x^k_2-\theta_2\tx_2-\theta_1\x_2^*\|^2_{\left(\alpha L_2+\frac{\beta\| \A_2^T \A_2\|}{\theta_1}\right)\I}\notag\\
&&-\frac{1}{2} \E_{i_k} \left(\|\x_2^{k+1}-(1-\theta_1-\theta_2)\x^k_2-\theta_2\tx_2-\theta_1\x_2^*\|^2_{\left(\alpha L_2+\frac{\beta\| \A_2^T \A_2\|}{\theta_1}\right)\I}\right)\notag.
\end{eqnarray}
So Lemma~1 is proved.
\\\\\\
\bfseries  Proof of Step 5: \mdseries

Taking expectation over the first $k$ iterations  for Eq.~\eqref{anns1} and diving $\theta_{1}$ on sides of it, we obtain:
\begin{eqnarray}
&&\!\!\!\!\!\!\!\!\!\!\!\frac{1}{\theta_{1}}\E\left[L(\x^{k+1}_1,\x^{k+1}_2,\olam^*)\right] - \frac{\theta_2}{\theta_{1}} L(\tx_1,\tx_2,\olam^*) -\frac{1-\theta_2 - \theta_1}{\theta_{1}}L(\x^{k}_1,\x^{k}_2,\olam^*)\\ 
&\leq& \frac{1}{2\beta}\left(\|\hlam^k-\olam^*\|^2- \E\left[\|\hlam^{k+1}-\olam^*\|^2\right] \right)  \notag\\
&&+\frac{\theta_{1}}{2}\|\frac{\y_1^{k}-(1-\theta_1-\theta_2)\x_1^{k}-\theta_2\tx_1}{\theta_1}-\x_1^*\|^2_{\left(L_1+\frac{\| \A_1^T \A_1\|}{\theta_1}\right)\I-\frac{\A_1^T\A_1}{\theta_1} }\notag\\
&&-\frac{\theta_{1}}{2}\E\left(\|\frac{\x^{k+1}_1-(1-\theta_1-\theta_2)\x_1^{k}-\theta_2\tx_1}{\theta_1}-\x_1^*\|^2_{\left(L_1+\frac{\| \A_1^T \A_1\|}{\theta_1}\right)\I-\frac{\A_1^T\A_1}{\theta_1} }\right)\notag\\
&&+ \frac{\theta_{1}}{2} \|\frac{\y_2^{k}-(1-\theta_1-\theta_2)\x^k_2-\theta_2\tx_2}{\theta_1}-\x_2^*\|^2_{\left(\alpha L_2+\frac{\| \A_2^T \A_2\|}{\theta_1}\right)\I}\notag\\
&&-\frac{\theta_{1}}{2} \E \left(\|\frac{\x_2^{k+1}-(1-\theta_1-\theta_2)\x^k_2-\theta_2\tx_2}{\theta_1}-\x_2^*\|^2_{\left(\alpha L_2+\frac{\| \A_2^T \A_2\|}{\theta_1}\right)\I}\right)\notag,
\end{eqnarray}
the expectation is taken under the condition that  randomness in the first $s$ epochs are
fixed. Since
\begin{eqnarray}
\y^{k} = \x^{k} +  (1-\theta_{1}-\theta_2)(\x^{k} - \x^{k-1}), \quad k\geq 1 \notag,
\end{eqnarray}
we obtain:
\begin{eqnarray}\label{fis}
&&\!\!\!\frac{1}{\theta_{1}}\E\left[L(\x^{k+1}_1,\x^{k+1}_2,\olam^*)\right] - \frac{\theta_2}{\theta_{1}} L(\tx_1,\tx_2,\olam^*) -\frac{1-\theta_2 - \theta_1}{\theta_{1}}L(\x^{k}_1,\x^{k}_2,\olam^*)\\ 
&\leq& \frac{1}{2\beta}\left(\|\hlam^k-\olam^*\|^2- \E\left[\|\hlam^{k+1}-\olam^*\|^2\right] \right)  \notag\\
&&+\frac{\theta_{1}}{2}\|\frac{\x_1^{k}-(1-\theta_1-\theta_2)\x_1^{k-1}-\theta_2\tx_1}{\theta_1}-\x_1^*\|^2_{\left(L_1+\frac{\| \A_1^T \A_1\|}{\theta_1}\right)\I-\frac{\A_1^T\A_1}{\theta_1} }\notag\\
&&-\frac{\theta_{1}}{2}\E\left(\|\frac{\x^{k+1}_1-(1-\theta_1-\theta_2)\x_1^{k}-\theta_2\tx_1}{\theta_1}-\x_1^*\|^2_{\left(L_1+\frac{\| \A_1^T \A_1\|}{\theta_1}\right)\I-\frac{\A_1^T\A_1}{\theta_1} }\right)\notag\\
&&+ \frac{\theta_{1}}{2} \|\frac{\x_2^{k}-(1-\theta_1-\theta_2)\x^{k-1}_2-\theta_2\tx_2}{\theta_1}-\x_2^*\|^2_{\left(\alpha L_2+\frac{\| \A_2^T \A_2\|}{\theta_1}\right)\I}\notag\\
&&-\frac{\theta_{1}}{2} \E \left(\|\frac{\x_2^{k+1}-(1-\theta_1-\theta_2)\x^k_2-\theta_2\tx_2}{\theta_1}-\x_2^*\|^2_{\left(\alpha L_2+\frac{\| \A_2^T \A_2\|}{\theta_1}\right)\I}\right), \quad k\geq 1 \notag.
\end{eqnarray}

Adding the subscript $s$ and taking expectation on the first $s$ epoches, and then  summing Eq.~\eqref{fis} with $k$ from $0$ to $m-1$, we have
\begin{eqnarray}\label{firstsum}
&&\frac{1}{\theta_{1,s}}\E\left(L(\x^{m}_s,\olam^*)-L(\x^*,\olam^*)\right)+ \frac{\theta_{2}+\theta_{1,s}}{\theta_{1,s}}\sum_{k=1}^{m-1} \E\left(L(\x^{k}_s,\olam^*)-L(\x^*,\olam^*)\right)\notag\\
&\overset{a}\leq&   \frac{1-\theta_{1,s}-\theta_2}{\theta_{1,s}}\E\left(L(\x^{m}_{s-1},\olam^*)-L(\x^*,\olam^*)\right)+ \frac{m\theta_{2}}{\theta_{1,s}}\E\left(L(\tx_{s},\olam^*)-L(\x^*,\olam^*)\right)\notag\\
&&+\frac{1}{2}\E\| \frac{ \y^{0}_{s,1}-\theta_2\tx_{s,1}-(1-\theta_{1,s}-\theta_{2})\x^{0}_{s,1}}{\theta_{1,s}}-\x^*_1   \|^2_{\left(\theta_{1,s}L_1+\| \A_1^T \A_1\|\right)\I-\A_1^T\A_1}\notag\\
&&-\frac{1}{2}\E\| \frac{ \x^{m}_{s,1}-\theta_2\tx_{s,1}-(1-\theta_{1,s}-\theta_{2})\x^{m-1}_{s,1}}{\theta_{1,s}}-\x^*_1   \|^2_{\left(\theta_{1,s}L_1+\| \A_1^T \A_1\|\right)\I-\A_1^T\A_1}\notag\\
&&+\frac{1}{2}\E\| \frac{ \y^{0}_{s,2}-\theta_2\tx_{s,2}-(1-\theta_{1,s}-\theta_{2})\x^{0}_{s,2}}{\theta_{1,s}}-\x^*_2   \|^2_{\left(\alpha \theta_{1,s}L_2+\| \A_2^T \A_2\|\right)\I}\notag\\
&&-\frac{1}{2}\E\| \frac{ \x^{m}_{s,2}-\theta_2\tx_{s,2}-(1-\theta_{1,s}-\theta_{2})\x^{m-1}_{s,2}}{\theta_{1,s}}-\x^*_2   \|^2_{\left(\alpha \theta_{1,s}L_2+\| \A_2^T \A_2\|\right)\I}\notag\\
&& +\frac{1}{2\beta}\left(\E\|\hlam^0_s-\olam^*\|^2- \E\left[\|\hlam^{m}_s-\olam^*\|^2\right] \right)\notag\\
&\overset{b}\leq&   \frac{1-\theta_{1,s}-(\tau-1)\theta_{1,{s}}}{\theta_{1,s}}\E\left(L(\x^{m}_{s-1},\olam^*)-L(\x^*,\olam^*)\right)+ \frac{\theta_{2}+\frac{\tau-1}{m-1}\theta_{1,{s}}}{\theta_{1,s}}\sum_{k=1}^{m-1}\E\left(L(\x^{k}_{s-1},\olam^*)-L(\x^*,\olam^*)\right)\notag\\
&&+\frac{1}{2}\E\| \frac{ \y^{0}_{s,1}-\theta_2\tx_{s,1}-(1-\theta_{1,s}-\theta_{2})\x^{0}_{s,1}}{\theta_{1,s}}-\x^*_1   \|^2_{\left(\theta_{1,s}L_1+\| \A_1^T \A_1\|\right)\I-\A_1^T\A_1}\notag\\
&&-\frac{1}{2}\E\| \frac{ \x^{m}_{s,1}-\theta_2\tx_{s,1}-(1-\theta_{1,s}-\theta_{2})\x^{m-1}_{s,1}}{\theta_{1,s}}-\x^*_1   \|^2_{\left(\theta_{1,s}L_1+\| \A_1^T \A_1\|\right)\I-\A_1^T\A_1}\notag\\
&&+\frac{1}{2}\E\| \frac{ \y^{0}_{s,2}-\theta_2\tx_{s,2}-(1-\theta_{1,s}-\theta_{2})\x^{0}_{s,2}}{\theta_{1,s}}-\x^*_2   \|^2_{\left(\alpha \theta_{1,s}L_2+\| \A_2^T \A_2\|\right)\I}\notag\\
&&-\frac{1}{2}\E\| \frac{ \x^{m}_{s,2}-\theta_2\tx_{s,2}-(1-\theta_{1,s}-\theta_{2})\x^{m-1}_{s,2}}{\theta_{1,s}}-\x^*_2   \|^2_{\left(\alpha \theta_{1,s}L_2+\| \A_2^T \A_2\|\right)\I}\notag\\
&& +\frac{1}{2\beta}\left(\E\|\hlam^0_s-\olam^*\|^2- \E\left[\|\hlam^{m}_s-\olam^*\|^2\right] \right),
\end{eqnarray}
where  we use $L(\x^k_s,\olam^*)$ and $L(\tx_s,\olam^*)$ to denote $L(\x^k_{s,1},  \x^k_{s,2},\olam^*)$ and $L(\tx_{s,1},\tx_{s,2}, \olam^*)$, respectively; the equality $ \overset{a}\leq$ uses $\x^m_{s-1}=\x^0_s$; the equality $ \overset{b}\leq$ uses the fact that 
\begin{eqnarray}
&&mL(\tx_s,\olam^*)\notag\\
&=&mL\left(  \frac{1}{m}\left(\left[1-\frac{(\tau-1)\theta_{1,{s}}}{\theta_2} \right]\x^m_{s-1}+\left[1+\frac{(\tau-1)\theta_{1,{s}}}{(m-1)\theta_2}\right]\sum_{k=1}^{m-1}\x^k_{s-1}\right),\olam^*\right)\notag\\
&\leq&\left[1-\frac{(\tau-1)\theta_{1,{s}}}{\theta_2} \right]L(\x^m_{s-1},\olam^*)+\left[1+\frac{(\tau-1)\theta_{1,{s}}}{(m-1)\theta_2}\right]\sum_{k=1}^{m-1}L(\x^k_{s-1},\olam^*),
\end{eqnarray}
since $L(\x,\olam^*)$ is convex for $\x$. Then for $\theta_{1,s}$ and $\theta_2$, we have
\begin{eqnarray}\label{temp1}
\frac{1}{\theta_{1,{s}}}=\frac{1-\tau\theta_{1,{s+1}}}{\theta_{1,{s+1}}}, \quad s\geq 0,
\end{eqnarray}
and 
\begin{eqnarray}\label{temp2}
\frac{\theta_2+\theta_{1,{s}}}{\theta_{1,{s}}}=\frac{\theta_2}{\theta_{1,{s+1}}}-\tau\theta_2+1=\frac{\theta_{2}+\frac{\tau-1}{m-1}\theta_{1,{s+1}}}{\theta_{1,s+1}}, \quad s\geq 0.
\end{eqnarray}
Substituting Eq.~\eqref{temp1}  into the first term and Eq.~\eqref{temp2} into the second term of Eq.~\eqref{firstsum}, we obtain
\begin{eqnarray}\label{imm2}
&&\frac{1}{\theta_{1,s}}\E\left(L(\x^{m}_s,\olam^*)-L(\x^*,\olam^*)\right)+ \frac{\theta_{2}+\theta_{1,s}}{\theta_{1,s}}\sum_{k=1}^{m-1} \E\left(L(\x^{k}_s,\olam^*)-L(\x^*,\olam^*)\right)\notag\\
&\leq&   \frac{1}{\theta_{1,s-1}}\E\left(L(\x^{m}_{s-1},\olam^*)-L(\x^*,\olam^*)\right)+ \frac{\theta_2+\theta_{1,{s-1}}}{\theta_{1,s-1}}\sum_{k=1}^{m-1}\E\left(L(\x^{k}_{s-1},\olam^*)-L(\x^*,\olam^*)\right)\notag\\
&&+\frac{1}{2}\E\| \frac{ \y^{0}_{s,1}-\theta_2\tx_{s,1}-(1-\theta_{1,s}-\theta_{2})\x^{0}_{s,1}}{\theta_{1,s}}-\x^*_1   \|^2_{\left(\theta_{1,s}L_1+\| \A_1^T \A_1\|\right)\I-\A_1^T\A_1}\notag\\
&&-\frac{1}{2}\E\| \frac{ \x^{m}_{s,1}-\theta_2\tx_{s,1}-(1-\theta_{1,s}-\theta_{2})\x^{m-1}_{s,1}}{\theta_{1,s}}-\x^*_1   \|^2_{\left(\theta_{1,s}L_1+\| \A_1^T \A_1\|\right)\I-\A_1^T\A_1}\notag\\
&&+\frac{1}{2}\E\| \frac{ \y^{0}_{s,2}-\theta_2\tx_{s,2}-(1-\theta_{1,s}-\theta_{2})\x^{0}_{s,2}}{\theta_{1,s}}-\x^*_2   \|^2_{\left(\alpha \theta_{1,s}L_2+\| \A_2^T \A_2\|\right)\I}\notag\\
&&-\frac{1}{2}\E\| \frac{ \x^{m}_{s,2}-\theta_2\tx_{s,2}-(1-\theta_{1,s}-\theta_{2})\x^{m-1}_{s,2}}{\theta_{1,s}}-\x^*_2   \|^2_{\left(\alpha \theta_{1,s}L_2+\| \A_2^T \A_2\|\right)\I}\notag\\
&& +\frac{1}{2\beta}\left(\E\|\hlam^0_s-\olam^*\|^2- \E\left[\|\hlam^{m}_s-\olam^*\|^2\right] \right).
\end{eqnarray}\\\\
\bfseries  Proof of Theorem 1 \mdseries \\
When $k=0$, for 
\begin{eqnarray}
\y_{s+1}^0 = (1-\theta_2)\x^m_s +\theta_2 \tx_{s+1}  +\frac{\theta_{1,s+1}}{\theta_{1,s}}\left[(1-\theta_{1,s})\x^m_s-(1-\theta_{1,s}-\theta_2)\x^{m-1}_s -\theta_2 \tx_s   \right],
\end{eqnarray} 
we obtain
\begin{eqnarray}\label{fory}
\frac{ \x^{m}_s-\theta_2\tx_s-(1-\theta_{1,s}-\theta_{2})\x^{m-1}_s}{\theta_{1,s}} =\frac{ \y^{0}_{s+1}-\theta_2\tx_{s+1}-(1-\theta_{1,{s+1}}-\theta_{2})\x^{0}_{s+1}}{\theta_{1,s+1}}.
\end{eqnarray}
Substituting Eq.~\eqref{fory} into the third and the fifth terms in the right hand of Eq.~\eqref{imm2} and substituting Eq.~\eqref{lams1} into the last term in the right hand of Eq.~\eqref{imm2}, we obtain
\begin{eqnarray}\label{tech}
&&\frac{1}{\theta_{1,s}}\E\left(L(\x^{m}_s,\olam^*)-L(\x^*,\olam^*)\right)+ \frac{\theta_2+\theta_{1,{s}}}{\theta_{1,s}}\sum_{k=1}^{m-1} \E\left(L(\x^{k}_s,\olam^*)-L(\x^*,\olam^*)\right)\\
&\leq&   \frac{1}{\theta_{1,s-1}}\E\left(L(\x^{m}_{s-1},\olam^*)-L(\x^*,\olam^*)\right)+ \frac{\theta_2+\theta_{1,{s-1}}}{\theta_{1,s-1}}\sum_{k=1}^{m-1}\E\left(L(\x^{k}_{s-1},\olam^*)-L(\x^*,\olam^*)\right)\notag\\
&&+\frac{1}{2}\E\| \frac{ \x^{m}_{s-1,1}-\theta_2\tx_{s-1,1}-(1-\theta_{1,s-1}-\theta_{2})\x^{m-1}_{s-1,1}}{\theta_{1,s-1}}-\x^*_1   \|^2_{\left(\theta_{1,s}L_1+\| \A_1^T \A_1\|\right)\I-\A_1^T\A_1}\notag\\
&&-\frac{1}{2}\E\| \frac{ \x^{m}_{s,1}-\theta_2\tx_{s,1}-(1-\theta_{1,s}-\theta_{2})\x^{m-1}_{s,1}}{\theta_{1,s}}-\x^*_1   \|^2_{\left(\theta_{1,s}L_1+\| \A_1^T \A_1\|\right)\I-\A_1^T\A_1}\notag\\
&&+\frac{1}{2}\E\|  \frac{ \x^{m}_{s-1,2}-\theta_2\tx_{s-1,2}-(1-\theta_{1,s-1}-\theta_{2})\x^{m-1}_{s-1,2}}{\theta_{1,s-1}}-\x^*_2    \|^2_{\left(\alpha \theta_{1,s}L_2+\| \A_2^T \A_2\|\right)\I}\notag\\
&&-\frac{1}{2}\E\| \frac{ \x^{m}_{s,2}-\theta_2\tx_{s,2}-(1-\theta_{1,s}-\theta_{2})\x^{m-1}_{s,2}}{\theta_{1,s}}-\x^*_2   \|^2_{\left(\alpha \theta_{1,s}L_2+\| \A_2^T \A_2\|\right)\I}\notag\\
&& +\frac{1}{2\beta}\left(\E\|\hlam^m_{s-1}-\olam^*\|^2- \E\left[\|\hlam^{m}_s-\olam^*\|^2\right] \right), \quad s\geq 1, 
\end{eqnarray}

For  $\theta_{1,s-1}\geq \theta_{1,s}$, so $\|\x\|^2_{\theta_{1,s-1}L}\geq \|\x\|^2_{\theta_{1,s}L}$, we get
\begin{eqnarray}
&&\frac{1}{\theta_{1,s}}\E\left(L(\x^{m}_s,\olam^*)-L(\x^*,\olam^*)\right)+ \frac{\theta_2+\theta_{1,{s}}}{\theta_{1,s}}\sum_{k=1}^{m-1} \E\left(L(\x^{k}_s,\olam^*)-L(\x^*,\olam^*)\right)\\
&\leq&   \frac{1}{\theta_{1,s-1}}\E\left(L(\x^{m}_{s-1},\olam^*)-L(\x^*,\olam^*)\right)+ \frac{\theta_2+\theta_{1,{s-1}}}{\theta_{1,s-1}}\sum_{k=1}^{m-1}\E\left(L(\x^{k}_{s-1},\olam^*)-L(\x^*,\olam^*)\right)\notag\\
&&+\frac{1}{2}\E\| \frac{ \x^{m}_{s-1,1}-\theta_2\tx_{s-1,1}-(1-\theta_{1,s-1}-\theta_{2})\x^{m-1}_{s-1,1}}{\theta_{1,s-1}}-\x^*_1   \|^2_{\left(\theta_{1,s-1}L_1+\| \A_1^T \A_1\|\right)\I-\A_1^T\A_1}\notag\\
&&-\frac{1}{2}\E\| \frac{ \x^{m}_{s,1}-\theta_2\tx_{s,1}-(1-\theta_{1,s}-\theta_{2})\x^{m-1}_{s,1}}{\theta_{1,s}}-\x^*_1   \|^2_{\left(\theta_{1,s}L_1+\| \A_1^T \A_1\|\right)\I-\A_1^T\A_1}\notag\\
&&+\frac{1}{2}\E\|  \frac{ \x^{m}_{s-1,2}-\theta_2\tx_{s-1,2}-(1-\theta_{1,s-1}-\theta_{2})\x^{m-1}_{s-1,2}}{\theta_{1,s-1}}-\x^*_2    \|^2_{\left(\alpha \theta_{1,s-1}L_2+\| \A_2^T \A_2\|\right)\I}\notag\\
&&-\frac{1}{2}\E\| \frac{ \x^{m}_{s,2}-\theta_2\tx_{s,2}-(1-\theta_{1,s}-\theta_{2})\x^{m-1}_{s,2}}{\theta_{1,s}}-\x^*_2   \|^2_{\left(\alpha \theta_{1,s}L_2+\| \A_2^T \A_2\|\right)\I}\notag\\
&& +\frac{1}{2\beta}\left(\E\|\hlam^m_{s-1}-\olam^*\|^2- \E\left[\|\hlam^{m}_s-\olam^*\|^2\right] \right), \quad s\geq 1, \notag
\end{eqnarray}

When $s=0$, through Eq.~\eqref{imm2}, and using  that $\y^0_{0,1}=\tx_{0,1}= \x^0_{0,1}$ and $\y^0_{0,2}=\tx_{0,2} = \x^0_{0,2}$,  we obtain
\begin{eqnarray}
&&\frac{1}{\theta_{1,0}}\E\left(L(\x^{m}_0,\olam^*))-L(\x^*,\olam^*)\right)+ \frac{\theta_{1,{0}}+\theta_2}{\theta_{1,0}}\sum_{k=1}^{m-1} \E\left(L(\x^{k}_0,\olam^*)-L(\x^*,\olam^*)\right)\notag\\
&\leq&  \frac{1-\theta_{1,0}+(m-1)\theta_2}{\theta_{1,0}}\left(L(\x_{0},\olam^*))-L(\x^*,\olam^*)\right)\notag\\
&&+\frac{1}{2}\|\x^0_{0,1}-\x^*_1   \|^2_{\left(\theta_{1,0}L_1+\| \A_1^T \A_1\|\right)\I-\A_1^T\A_1}\notag\\
&&-\frac{1}{2}\E\| \frac{ \x^{m}_{0,1}-\theta_2\tx_{0,1}-(1-\theta_{1,0}-\theta_{2})\x^{m-1}_{0,1}}{\theta_{1,s=0}}-\x^*_1   \|^2_{\left(\theta_{1,0}L_1+\| \A_1^T \A_1\|\right)\I-\A_1^T\A_1}\notag\\
&&+\frac{1}{2}\| \x^0_{0,2}-\x^*_1  \|^2_{\left(\alpha \theta_{1,0}L_2+\| \A_2^T \A_2\|\right)\I}\notag\\
&&-\frac{1}{2}\E\| \frac{ \x^{m}_{0,2}-\theta_2\tx_{0,2}-(1-\theta_{1,0}-\theta_{2})\x^{m-1}_{0,2}}{\theta_{1,0}}-\x^*_2   \|^2_{\left(\alpha \theta_{1,0}L_2+\| \A_2^T \A_2\|\right)\I}\notag\\
&& +\frac{1}{2\beta}\left(\|\hlam^0_{0}-\olam^*\|^2- \E\left[\|\hlam^{m}_0-\olam^*\|^2\right] \right).
\end{eqnarray}
Summing $s$ from $0$ to $S-1$, we have the result that
\begin{eqnarray}\label{forL}
&&\frac{1}{\theta_{1,S}}\E\left(L(\x^{m}_S,\olam^*))-L(\x^*,\olam^*)\right)+ \frac{\theta_{1,{S}}+\theta_2}{\theta_{1,S}}\sum_{k=1}^{m-1} \E\left(L(\x^{k}_S,\olam^*)-L(\x^*,\olam^*)\right)\notag\\
&\leq&  \frac{1-\theta_{1,0}+(m-1)\theta_2}{\theta_{1,0}}\left(L(\x^0_{0},\olam^*))-L(\x^*,\olam^*)\right)\notag\\
&&   +\frac{1}{2}\|\x^0_{0,1}-\x^*_1   \|^2_{\left(\theta_{1,0}L_1+\| \A_1^T \A_1\|\right)\I-\A_1^T\A_1}+\frac{1}{2}\| \x^0_{0,2}-\x^*_2  \|^2_{\left(\alpha \theta_{1,0}L_2+\| \A_2^T \A_2\|\right)\I}\notag\\ 
&&+ \frac{1}{2\beta}\left(\|\hlam^0_{0}-\olam^*\|^2- \E\left[\|\hlam^{m}_S-\olam^*\|^2\right] \right)\notag\\
&&-\frac{1}{2}\E\| \frac{ \x^{m}_{S,1}-\theta_2\tx_{S,1}-(1-\theta_{1,s}-\theta_{2})\x^{m-1}_{S,1}}{\theta_{1,S}}-\x^*_1   \|^2_{\left(\theta_{1,S}L_1+\| \A_1^T \A_1\|\right)\I-\A_1^T\A_1}\notag\\
&&-\frac{1}{2}\E\| \frac{ \x^{m}_{S,2}-\theta_2\tx_{S,2}-(1-\theta_{1,S}-\theta_{2})\x^{m-1}_{s,2}}{\theta_{1,S}}-\x^*_2   \|^2_{\left(\alpha \theta_{1,S}L_2+\| \A_2^T \A_2\|\right)\I}\notag\\
&\leq&  \frac{1-\theta_{1,0}+(m-1)\theta_2}{\theta_{1,0}}\left(L(\x^0_{0},\olam^*))-L(\x^*,\olam^*)\right)\notag\\
&&   +\frac{1}{2}\|\x^0_{0,1}-\x^*_1   \|^2_{\left(\theta_{1,0}L_1+\| \A_1^T \A_1\|\right)\I-\A_1^T\A_1}+\frac{1}{2}\| \x^0_{0,2}-\x^*_2  \|^2_{\left(\alpha \theta_{1,0}L_2+\| \A_2^T \A_2\|\right)\I}\notag\\ 
&&+ \frac{1}{2\beta}\left(\|\hlam^0_{0}-\olam^*\|^2- \E\left[\|\hlam^{m}_S-\olam^*\|^2\right] \right).
\end{eqnarray}
Now we analyse $ \|\hlam^{m}_S-\olam^*\|^2 $. From Eq.~\eqref{lams1}, for $s\geq 1$, we have
\begin{eqnarray}\label{hlam222}
&&\hlam^{m}_s-\hlam^{m}_{s-1}=\hlam^{m}_s-\hlam^{0}_{s}= \sum_{k=1}^m \left(\hlam^{k}_s-\hlam^{k-1}_{s}\right)\notag\\
&\overset{a}=& \beta\sum_{k=1}^m \left( \frac{1}{\theta_{1,{s}}} \left(\A\x^k_s-\b\right) -  \frac{1-\theta_{1,{s}}-\theta_2}{\theta_{1,{s}}} \left(\A\x^{k-1}_s-\b\right) - \frac{\theta_2}{\theta_{1,{s}}} \left(\A\tx_s-\b\right)  \right)\notag\\
&\overset{b}=& \frac{\beta}{\theta_{1,s}}\left(\A\x^m_s-\b\right)+ \frac{\beta(\theta_2+\theta_{1,{s}})}{\theta_{1,s}}\sum_{k=1}^{m-1} \left(\A\x^k_s-\b\right)\notag\\
&& -\frac{\beta(1-\theta_{1,s}-\theta_2)}{\theta_{1,s}}\left(\A\x^m_{s-1}-\b\right)- \frac{m\beta\theta_2}{\theta_{1,s}} \left(\A\tx_{s-1}-\b\right)\notag\\
&\overset{c}=& \frac{\beta}{\theta_{1,s}}\left(\A\x^m_s-\b\right)+ \frac{\beta(\theta_2+\theta_{1,{s}})}{\theta_{1,s}}\sum_{k=1}^{m-1} \left(\A\x^k_s-\b\right)\notag\\
&&-\beta\left( \frac{1-\theta_{1,s}-(\tau-1)\theta_{1,{s}}}{\theta_{1,s}}\left(\A\x^m_{s-1}-\b\right)+ \frac{\theta_{2}+\frac{\tau}{m-1}\theta_{1,{s}}}{\theta_{1,s}}\sum_{k=1}^{m-1}\left(\A\x^k_{s-1}-\b\right)\right)\notag\\
&\overset{d}=& \frac{\beta}{\theta_{1,s}}\left(\A\x^m_s-\b\right)+ \frac{\beta(\theta_2+\theta_{1,{s}})}{\theta_{1,s}}\sum_{k=1}^{m-1} \left(\A\x^k_s-\b\right)\notag\\
&&-\frac{\beta}{\theta_{1,s-1}}\left(\A\x^m_{s-1}-\b\right)- \frac{\beta(\theta_2+\theta_{1,{s-1}})}{\theta_{1,s-1}}\sum_{k=1}^{m-1} \left(\A\x^k_{s-1}-\b\right),
\end{eqnarray}
where the equality $\overset{a}=$ uses Eq.~\eqref{hlamlist};   the equalities $\overset{b}=,\overset{c}=$, and $\overset{d}=$  are obtained through the same techniques of Eq.~\eqref{firstsum} and Eq.~\eqref{imm2}.
When $s = 0$, we can obtain 
\begin{eqnarray}\label{hlam3}
&&\hlam^{m}_0-\hlam^{0}_{0}= \sum_{k=1}^m \left(\hlam^{k}_0-\hlam^{k-1}_{0}\right)\\
&=& \sum_{k=1}^m \left( \frac{\beta}{\theta_{1,{0}}} \left(\A\x^k_0-\b\right) -  \frac{\beta(1-\theta_{1,{0}}-\theta_2)}{\theta_{1,{0}}} \left(\A\x^{k-1}_0-\b\right) - \frac{\theta_2\beta}{\theta_{1,{0}}} \left(\A\x^0_0-\b\right)  \right)\notag\\
&=& \frac{\beta}{\theta_{1,0}}\left(\A\x^m_0-\b\right)+ \frac{\beta(\theta_2+\theta_{1,{0}})}{\theta_{1,0}}\sum_{k=1}^{m-1} \left(\A\x^k_0-\b\right) - \frac{\beta(1-\theta_{1,0}+(m-1)\theta_2)}{\theta_{1,0}}\left(\A\x^0_0-\b  \right).\notag
\end{eqnarray}
Summing Eq.~\eqref{hlam222} with $s$ from $0$ to $S-1$, we have the result that
\begin{eqnarray}\label{hlam4}
&&\hlam^{m}_S-\olam^*= \hlam^{m}_S-\hlam^0_0 + \hlam^0_0 - \olam^*\notag\\
&\overset{a}=&  \frac{\beta}{\theta_{1,S}}\left(\A\x^m_S-\b\right)+ \frac{\beta(\theta_2+\theta_{1,{S}})}{\theta_{1,S}}\sum_{k=1}^{m-1} \left(\A\x^k_S-\b\right) - \frac{\beta\left(1-\theta_{1,0}+(m-1)\theta_2\right)}{\theta_{1,0}}\left(\A\x^0_0-\b  \right)\notag\\
&& +\tlam^{0}_0 +\frac{\beta(1-\theta_{1,{0}})}{\theta_{1,{0}}}\left(\A\x^0_{0}-\b \right)  - \olam^*\notag\\
&\overset{b}=&\frac{m\beta}{\theta_{1,{S}}}\left(\A\hat{\x}_S-\b  \right) +\tlam^0_0 -\frac{\beta(m-1)\theta_2}{\theta_{1,{0}}}\left( \A\x^0_0 -\b\right) -\olam^*.
\end{eqnarray}
where we have substituted Eq.~\eqref{hlam3} in the equality $\overset{a}=$; the equality $\overset{b}=$ uses the definition of $\hat{\x}_S$. Substituting Eq.~\eqref{hlam4} into Eq.~\eqref{forL}, we can obtain Theorem 1.
\\\\\\
\bfseries  Proof of Corollary 1 \mdseries 
\\ We set
\begin{eqnarray}
C_1&=& \frac{1-\theta_{1,0}+(m-1)\theta_2}{\theta_{1,0}}\left(F(\x^0_{0})-F(\x^*)  +\langle \olam^*, \A\x^0_0 -\b\rangle\right)\\
&&+\frac{1}{2\beta}\|\tlam^0_0 +\frac{\beta(1-\theta_{1,{0}})}{\theta_{1,{0}}}(\A\x^0_0-\b) -\olam^*  \|^2\notag\\
&&+\frac{1}{2}\|\x^0_{0,1}-\x^*_1   \|^2_{\left(\theta_{1,0}L_1+\| \A_1^T \A_1\|\right)\I-\A_1^T\A_1}+\frac{1}{2}\| \x^0_{0,2}-\x^*_2  \|^2_{\left((1+\frac{1}{b\theta_2}) \theta_{1,0}L_2\right)\I+\| \A_2^T \A_2\|}.\notag
\end{eqnarray}
Since $F(\x)$ is convex,  
$$F(\hat{\x}_{S})-F(\x^*) +\langle \olam^* ,\A\hat{\x}_S -\b\rangle \geq0 .$$
Taking expectation, we obtain:
$$\E \left(F(\hat{\x}_{S})-F(\x^*) +\langle \olam^* ,\A\hat{\x}_S -\b\rangle \right)\geq0 .$$
Then from Theorem 1, we obtain 
\begin{eqnarray}
\E\left(F(\hat{\x}_{S})-F(\x^*) +\langle \olam^* ,\A\hat{\x}_S -\b\rangle 
\right)\leq \frac{C_1}{m}\theta_{1,{S}},
\end{eqnarray}
and
\begin{eqnarray}
\E\|   \frac{m\beta}{\theta_{1,{S}}}\left(\A\hat{\x}_S-\b  \right) +\olam^0_0 -\frac{\beta(m-1)\theta_2}{\theta_{1,{0}}}\left( \A\x_0 -\b\right) -\olam^*  \|^2 \leq   2\beta C_1,
\end{eqnarray}
So
\begin{eqnarray}
\E\|   \frac{m\beta}{\theta_{1,{S}}}\left(\A\hat{\x}_S-\b  \right) +\olam^0_0 -\frac{\beta(m-1)\theta_2}{\theta_{1,{0}}}\left( \A\x_0 -\b\right) -\olam^*  \| \leq   \sqrt{2\beta C_1},
\end{eqnarray}
where we use the fact that $0\leq\E\|\xi-\E(\xi)\|^2=\E\|\xi\|^2-\|\E\xi\|^2$. Since $\|\mathbf{a}-\mathbf{b}  \|\geq \|\mathbf{a} \| -\|\mathbf{b} \|$, we obtain 
\begin{eqnarray}
\E\|   \frac{m\beta}{\theta_{1,{S}}}\left(\A\hat{\x}_S-\b  \right)\|\leq C_2, 
\end{eqnarray}
where  $C_2=\sqrt{2\beta C_1}+ \| \olam^0_0 -\frac{\beta(m-1)\theta_2}{\theta_{1,{0}}}\left( \A\x_0 -\b\right) -\olam^* \|$.
Thus 
\begin{eqnarray}
\E\|\A\hat{\x}_S- \b\| \leq \frac{C_2 }{m\beta}\theta_{1,{S}} = O(\frac{1}{S}).
\end{eqnarray}
For  $\E \left(F(\hat{\x}_{S})-F(\x^*) +\langle \olam^* ,\A\hat{\x}_S -\b\rangle \right)\geq0$, we obtain
\begin{eqnarray}
-\E\|\olam^*\|\|\A\hat{\x}_S -\b\| \leq\E \left( F(\hat{\x}_{S})-F(\x^*) \right)\leq \frac{C_1}{m}\theta_{1,{S}}+\E\|\olam^*\|\|\A\hat{\x}_S -\b\|.
\end{eqnarray}
So 
\begin{eqnarray}
\E|F(\hat{\x}_{S})-F(\x^*)| \leq O(\frac{1}{S}).
\end{eqnarray}
This ends the proof.

\section{Experiments}
\subsection{Lasso Problems}
We compare our method with (1) STOC-ADMM~\cite{STOC-ADMM}, (2) SVRG-ADMM~\cite{SVRG-ADMM}, (3) OPT-SADMM~\cite{OPT-SADMM}, (4) SAG-ADMM~\cite{SAG-ADMM}. We implement those algorithms as follows:
\begin{itemize}
	\item   STOC-ADMM~\cite{STOC-ADMM}. The step size for STOC-ADMM  $\gamma = 1/(L_2 +\sigma k^{\frac{1}{2}}+\beta\|\A^T\A\|)$. We set $\beta_s = \min(10,\rho^s \beta_0)$ and tune $\sigma$ from  $\{10^{-5},10^{-4},10^{-3}\}$.
	\item   OPT-ADMM~\cite{OPT-SADMM}. The step size for OPT-ADMM $\gamma = 1/(L_2 +\sigma k^{\frac{3}{2}}+\beta\|\A^T\A\|)$. We set $\beta_s = \min(10,\rho^s \beta_0)$ and tune $\sigma$ from  $\{10^{-7},10^{-6},10^{-5}\}$.
	\item   SVRG-ADMM~\cite{SVRG-ADMM}. The step size for SVRG-ADMM  $\gamma = 1/(L_2 +\beta\|\A^T\A\|)$. We set $\beta_s = \min(10,\rho^s \beta_0)$.
	\item   SAG-ADMM~\cite{SAG-ADMM}. The step size for SAG-ADMM $\gamma = 1/(L_2 +\beta)$. We set $\beta_s = \min(10,\rho^s \beta_0)$.
	\item   ACC-SADMM~(ours). The step size for ACC-SADMM is $\gamma = 1/(L_2(1+\frac{2}{b}) +\frac{\beta_0}{\theta_{1,s}}\|\A^T\A\|)$. 
\end{itemize}
For all the other algorithms, we tune $\rho$ from $\{1,1.05,1.1,1.3\}$. And we tune  $\beta_0$ from $\{10^{-4},10^{-3},10^{-2},10^{-1}\}$. For the original Lasso problem~(Eq.(27) in the paper), $L_2=1$. For the Graph-Guided Fused Lasso problem~(Eq.(28) in the paper), $L_2$ is tuned from $\{1\times 10^k,2\times 10^k,5\times 10^k|-5\leq k\leq -1, k\in \mathcal{Z} \}$ to obtain the best step size for each algorithm.  

In experiment, we first fix $\sigma=0$ and $\rho=1$ and then tune the parameters $\beta_0$ and $L_2$ based on the first $10$ data passes. Then we retune the parameters for $\sigma$ and $\rho$. For some algorithms, there are $4$ parameters to tune. However, we find that the major factors of the speed for the algorithms are $\beta_0$ and $L_2$.

Fig.~\ref{experimentsss} shows more experimental results with fixed $L_2=0.01$ for the original Lasso problem~(Eq.(27) in the paper) and the Graph-Guided Fused Lasso problem~(Eq.(28) in the paper) on the a9a and mnist datasets. Our method is also faster than other algorithms. Table~\ref{memoryss} reports the memory costs of all algorithms.
\begin{figure}[!h]
	\subfigure[a9a-original Lasso]{ 
		{\label{fig:1}} %% label for first subfigure 
		\includegraphics[width=0.45\linewidth]{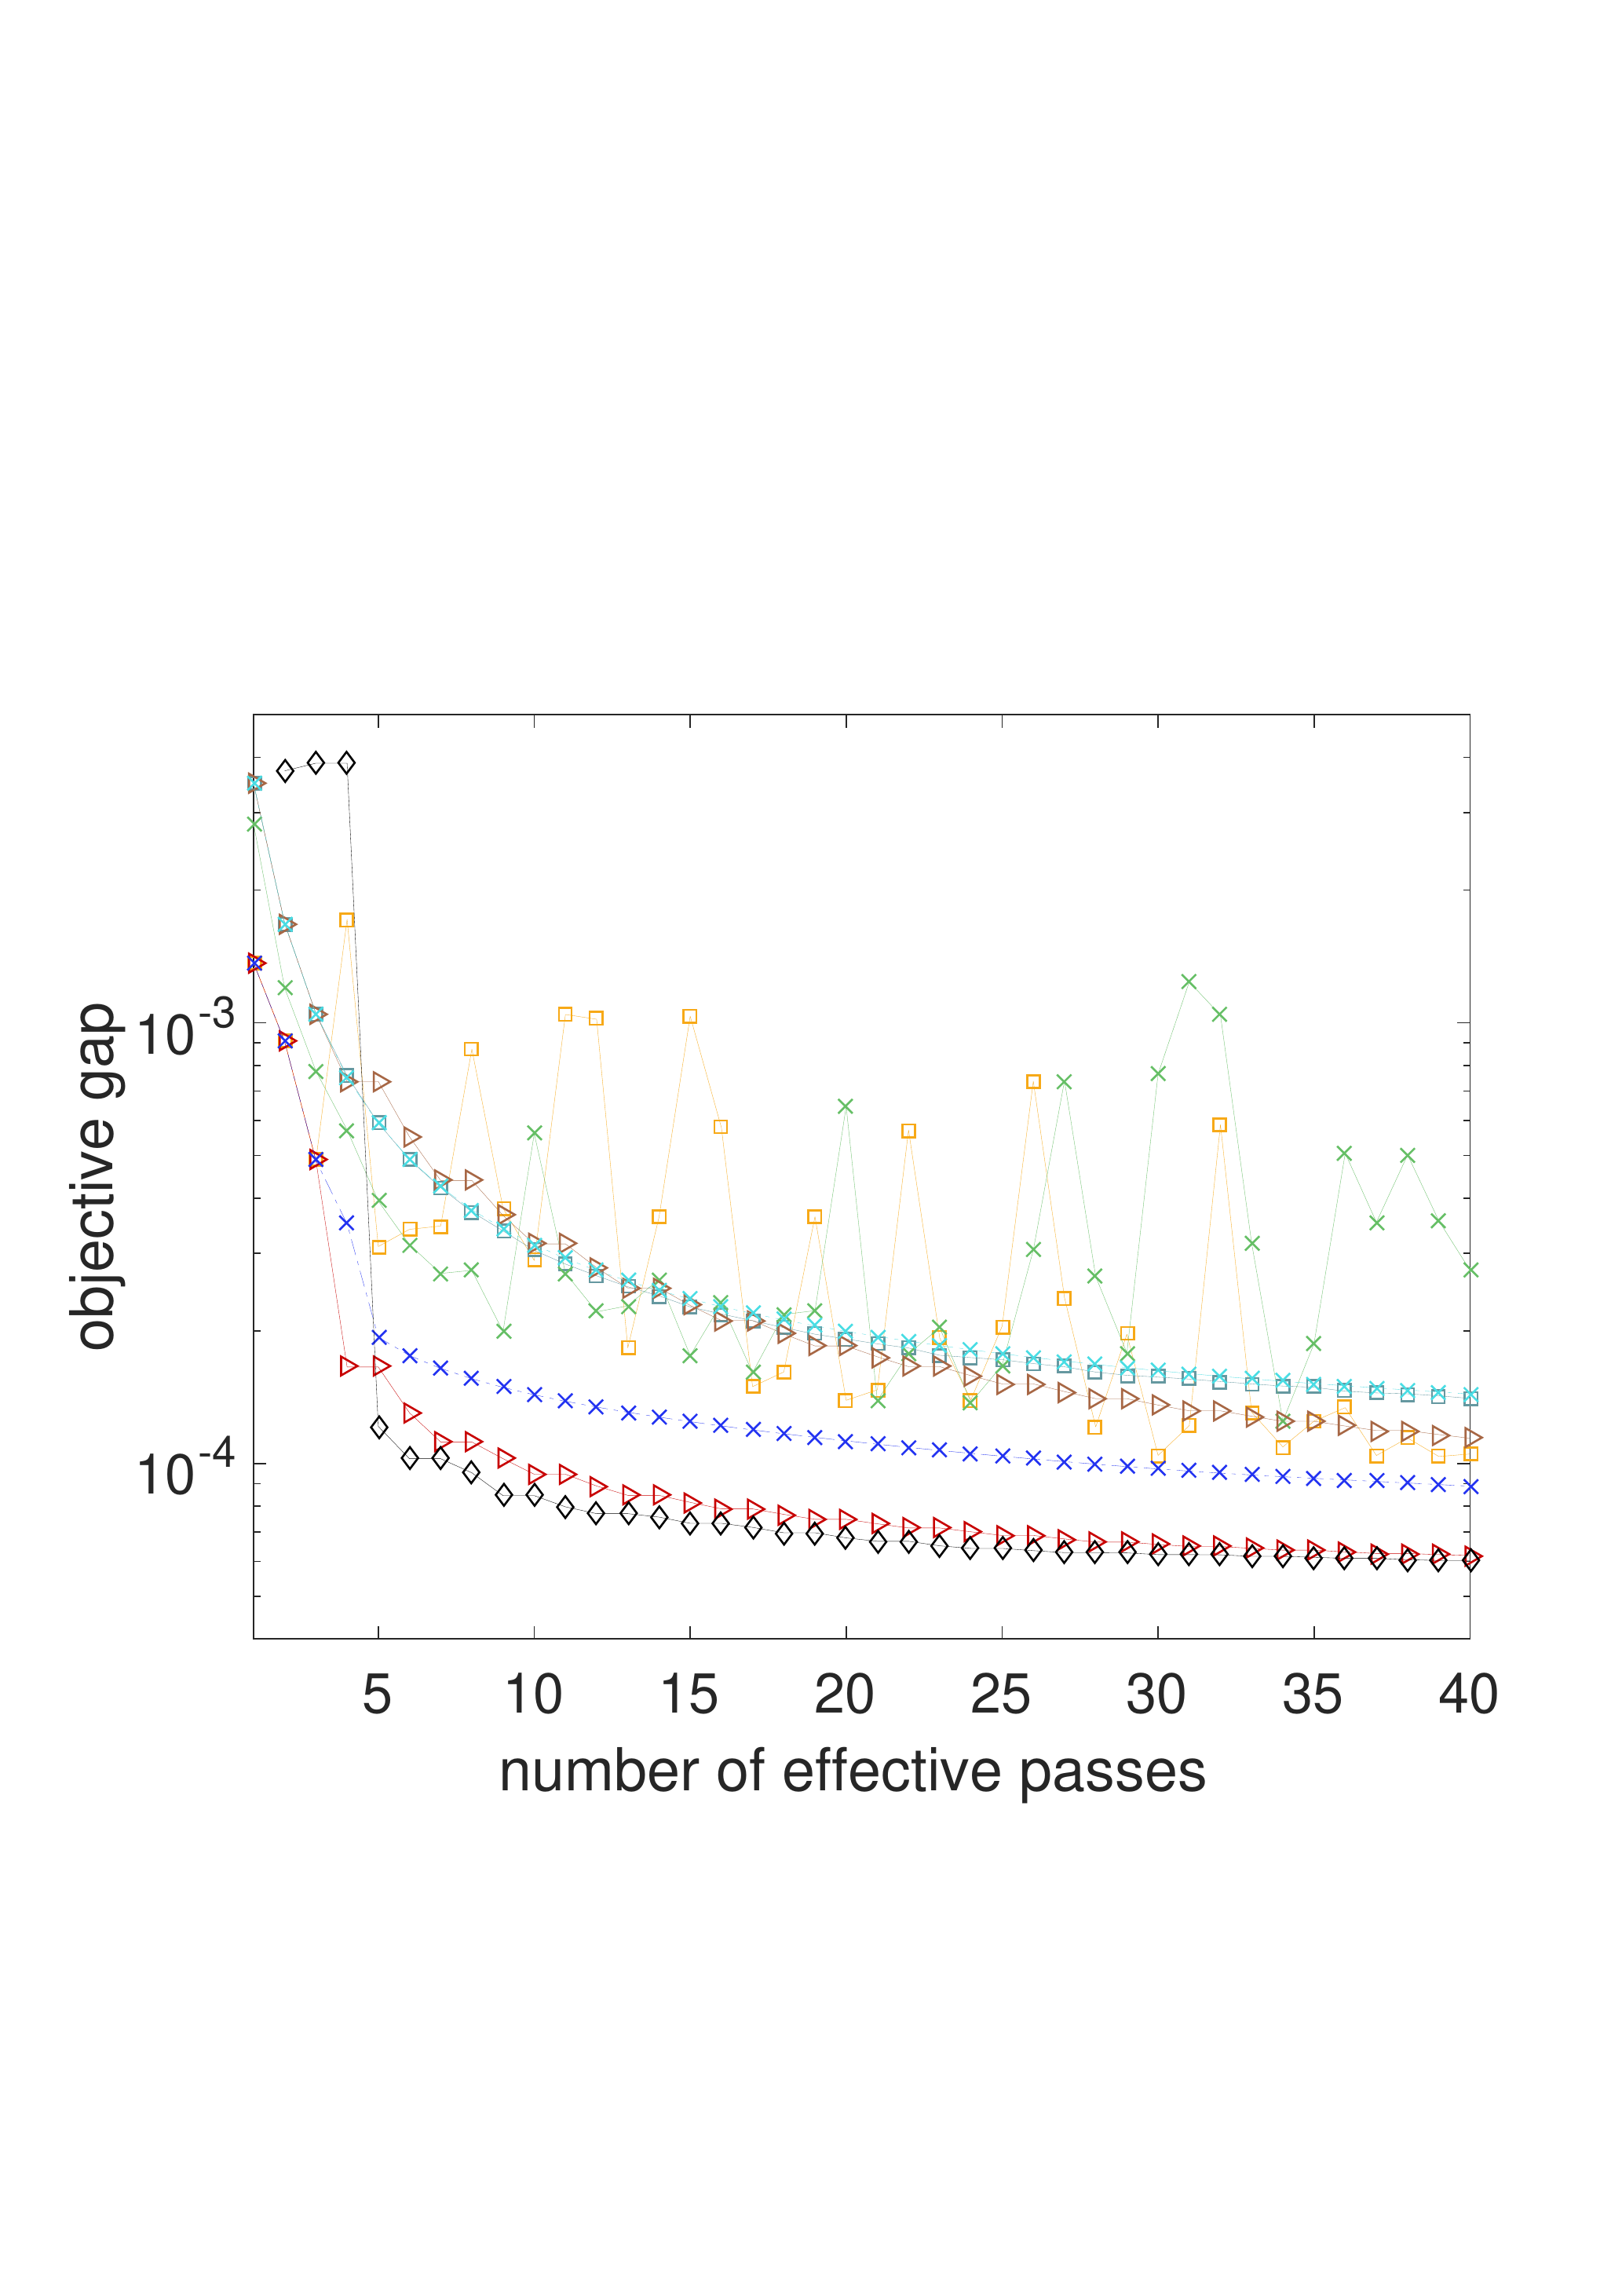}} 
%	\hspace{-0.1in} 
	\subfigure[mnist-original Lasso]{ 
		\label{fig:2} %% label for second subfigure 
		\includegraphics[width=0.45\linewidth]{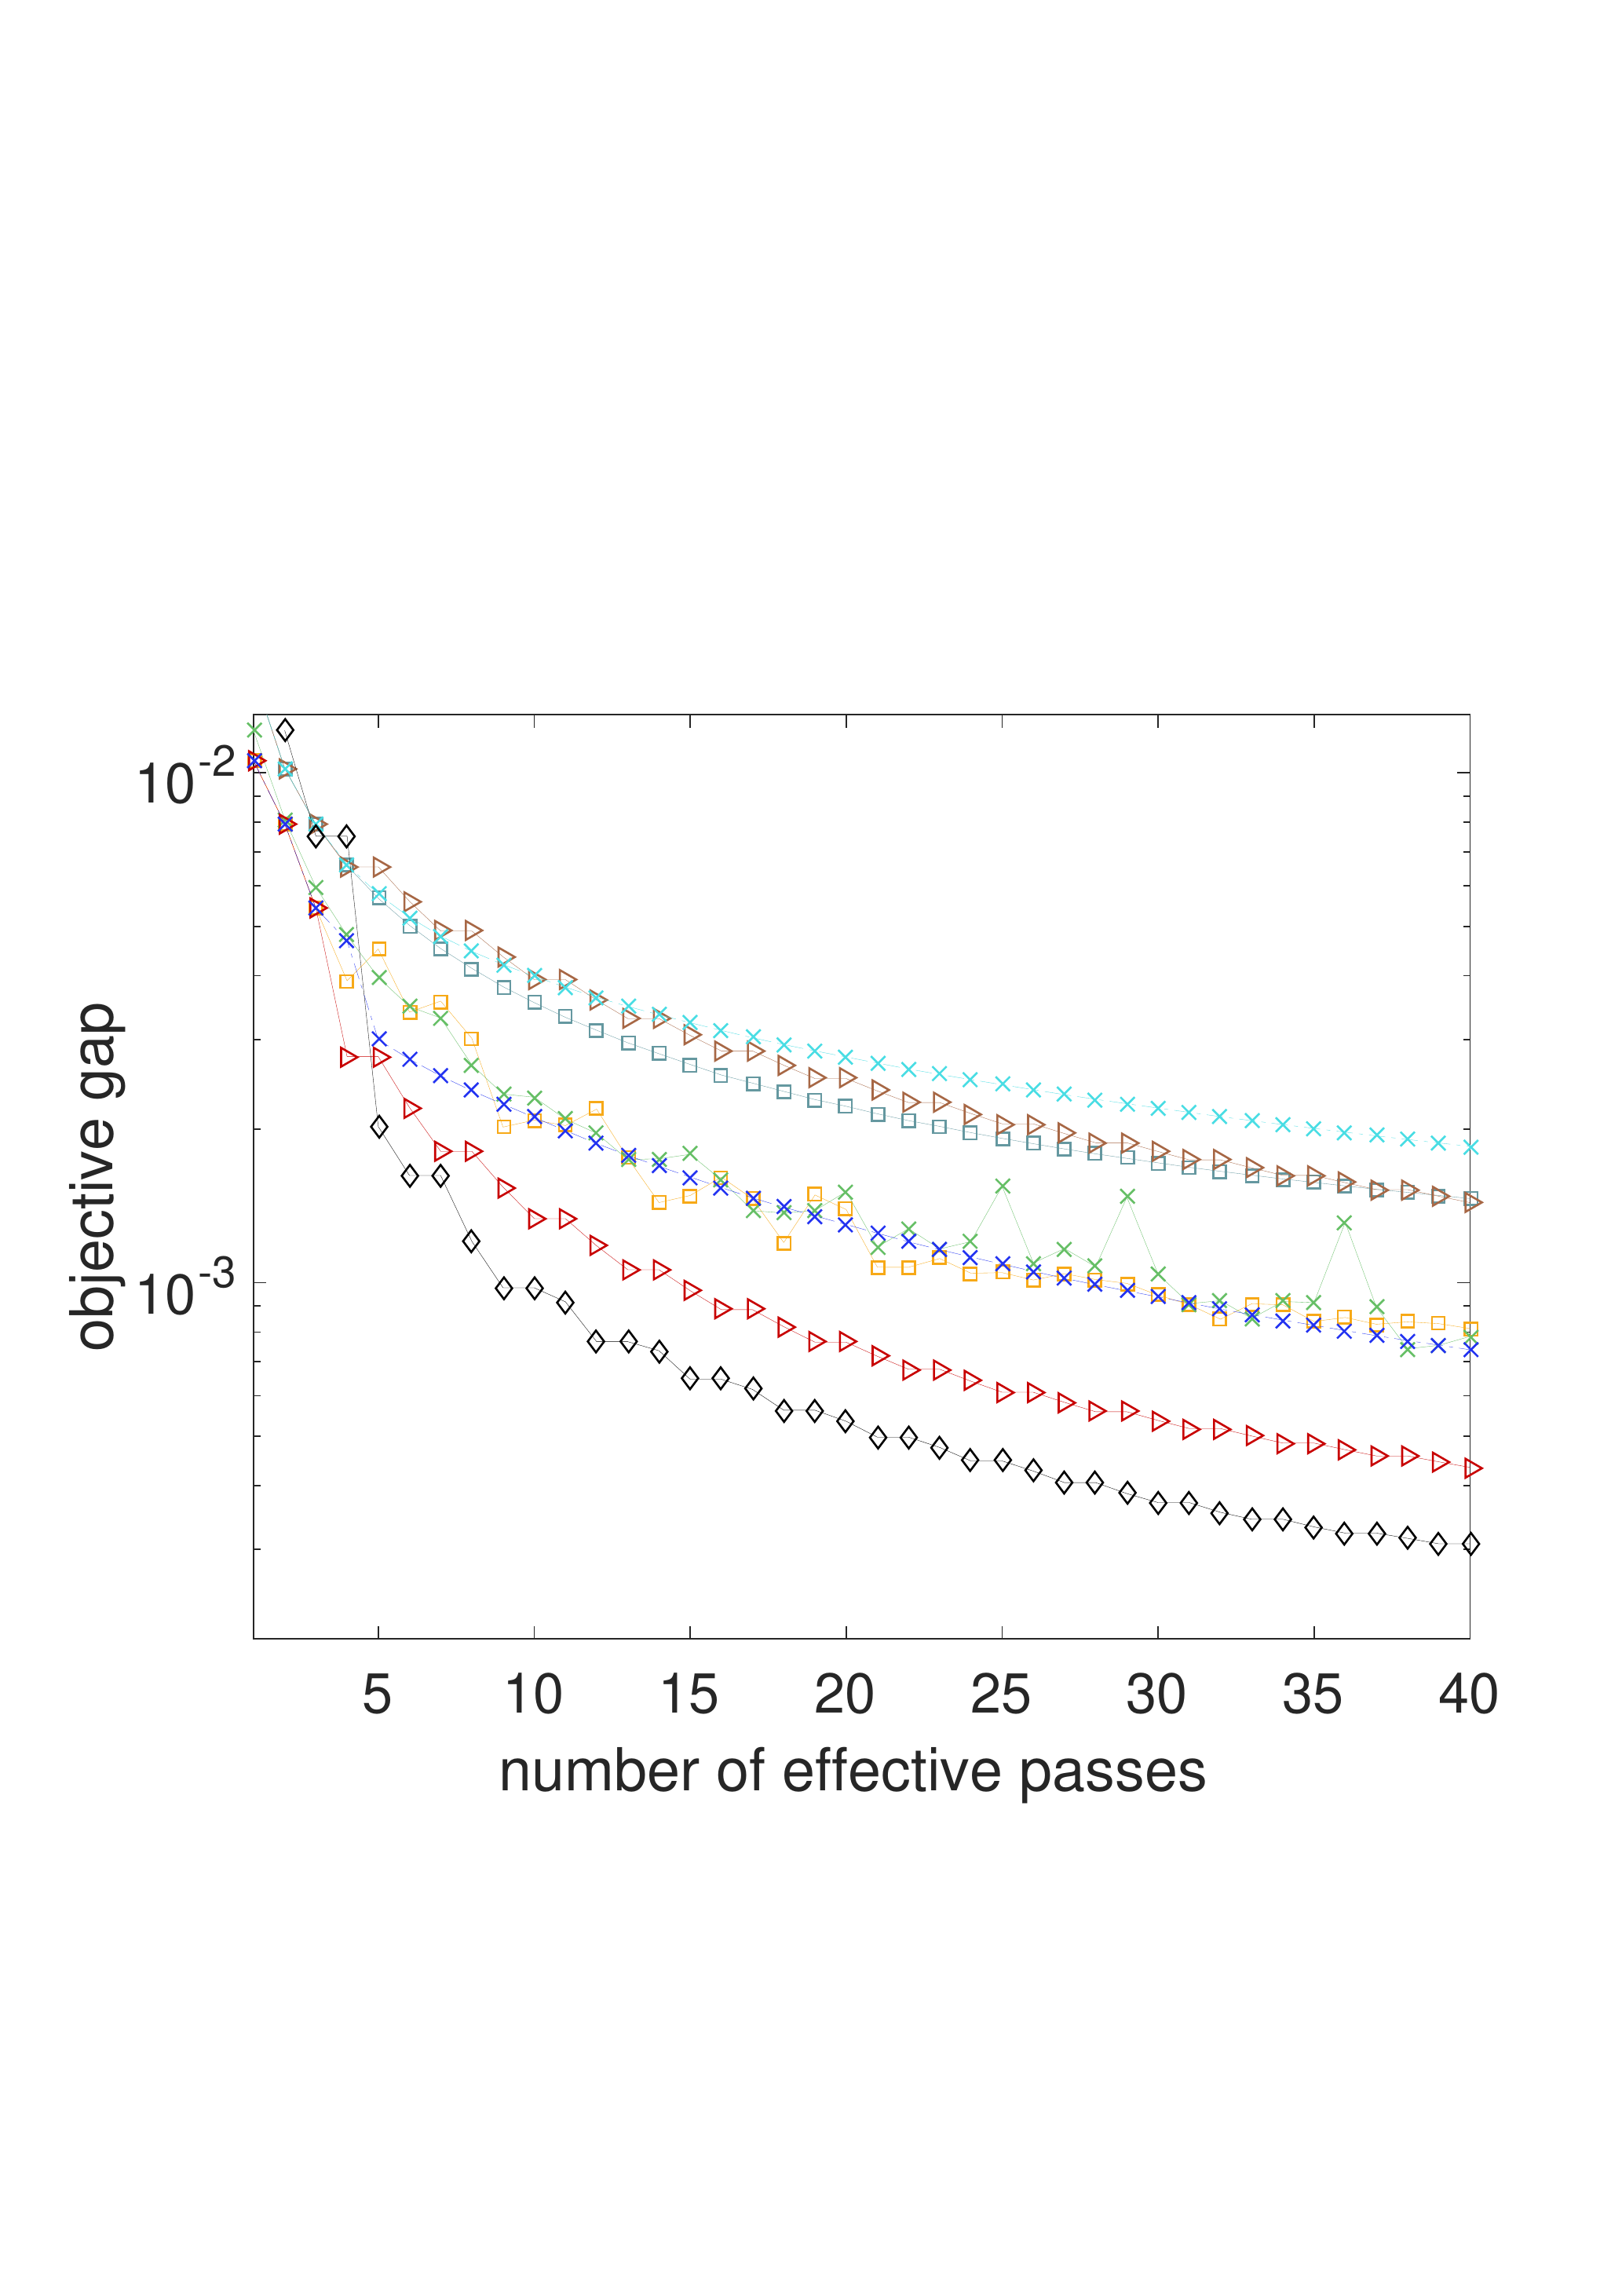}  
	}    
%	\hspace{-0.1in} 
	\subfigure[a9a-Graph-Guided Lasso]{ 
		\label{fig:3} %% label for second subfigure 
		\includegraphics[width=0.45\linewidth]{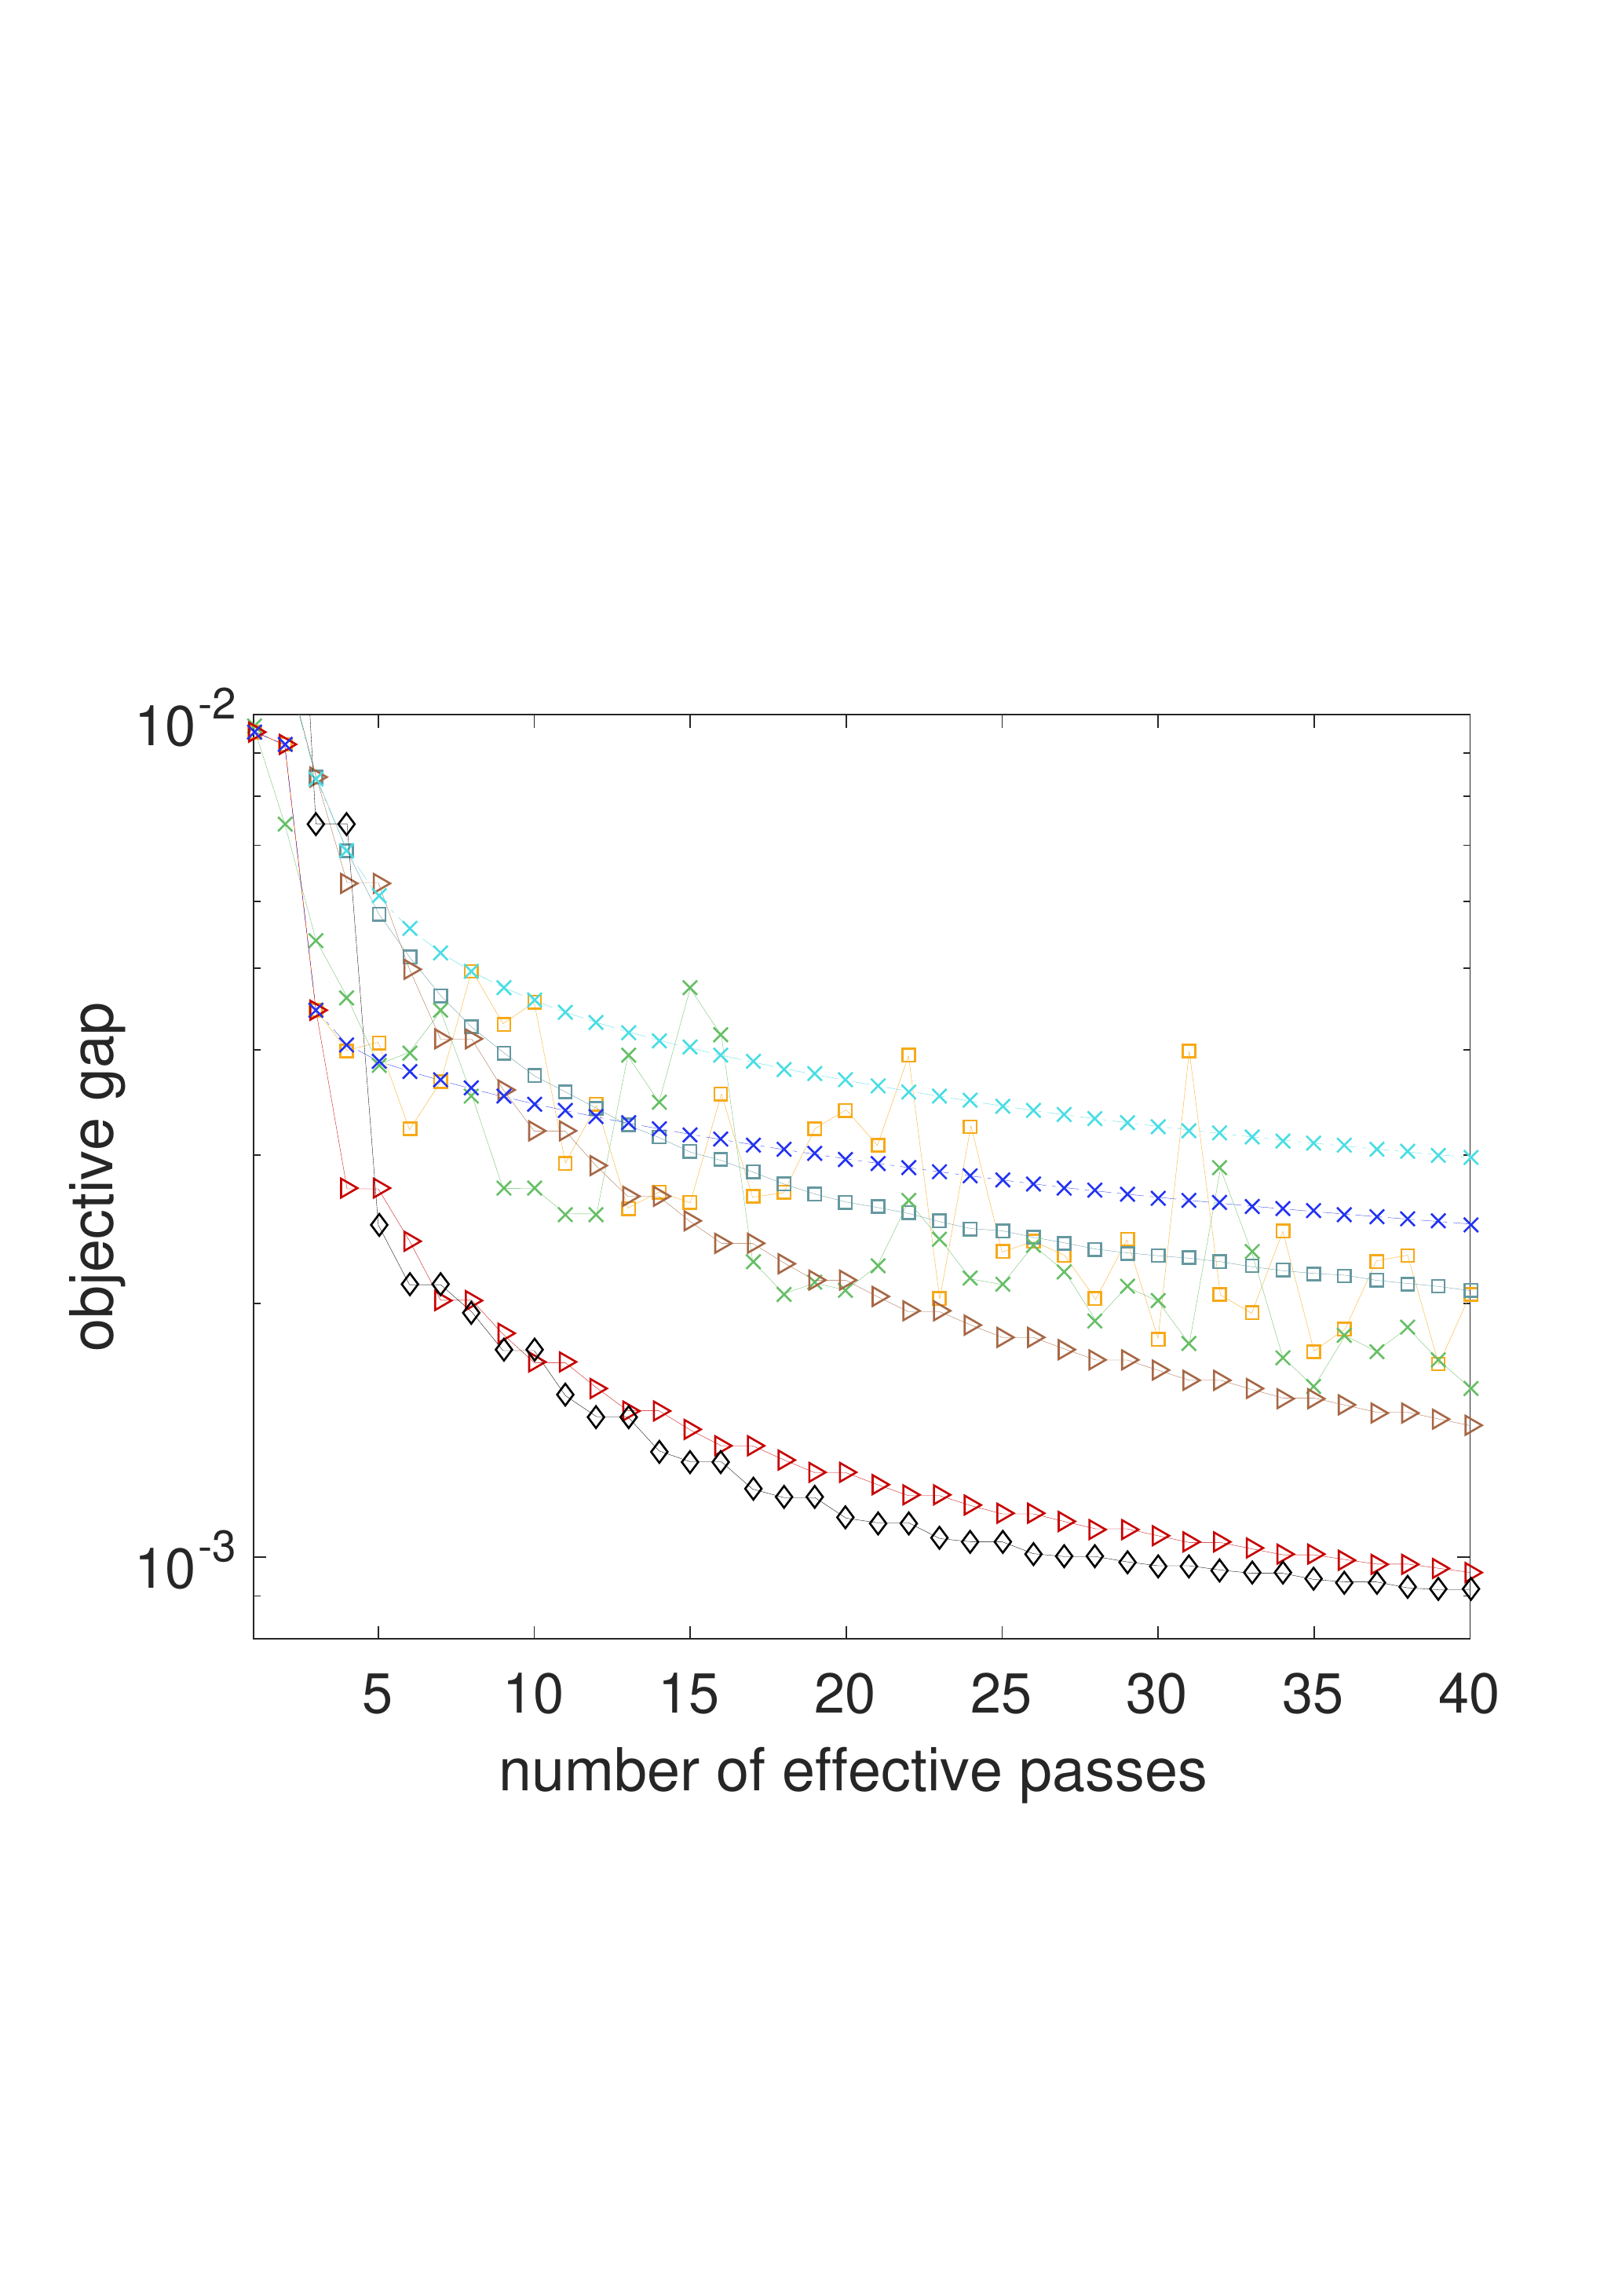}}  
%	\hspace{-0.1in} 
	\subfigure[mnist-Graph-Guided Lasso]{ 
		\label{fig:4} %% label for second subfigure 
		\includegraphics[width=0.45\linewidth]{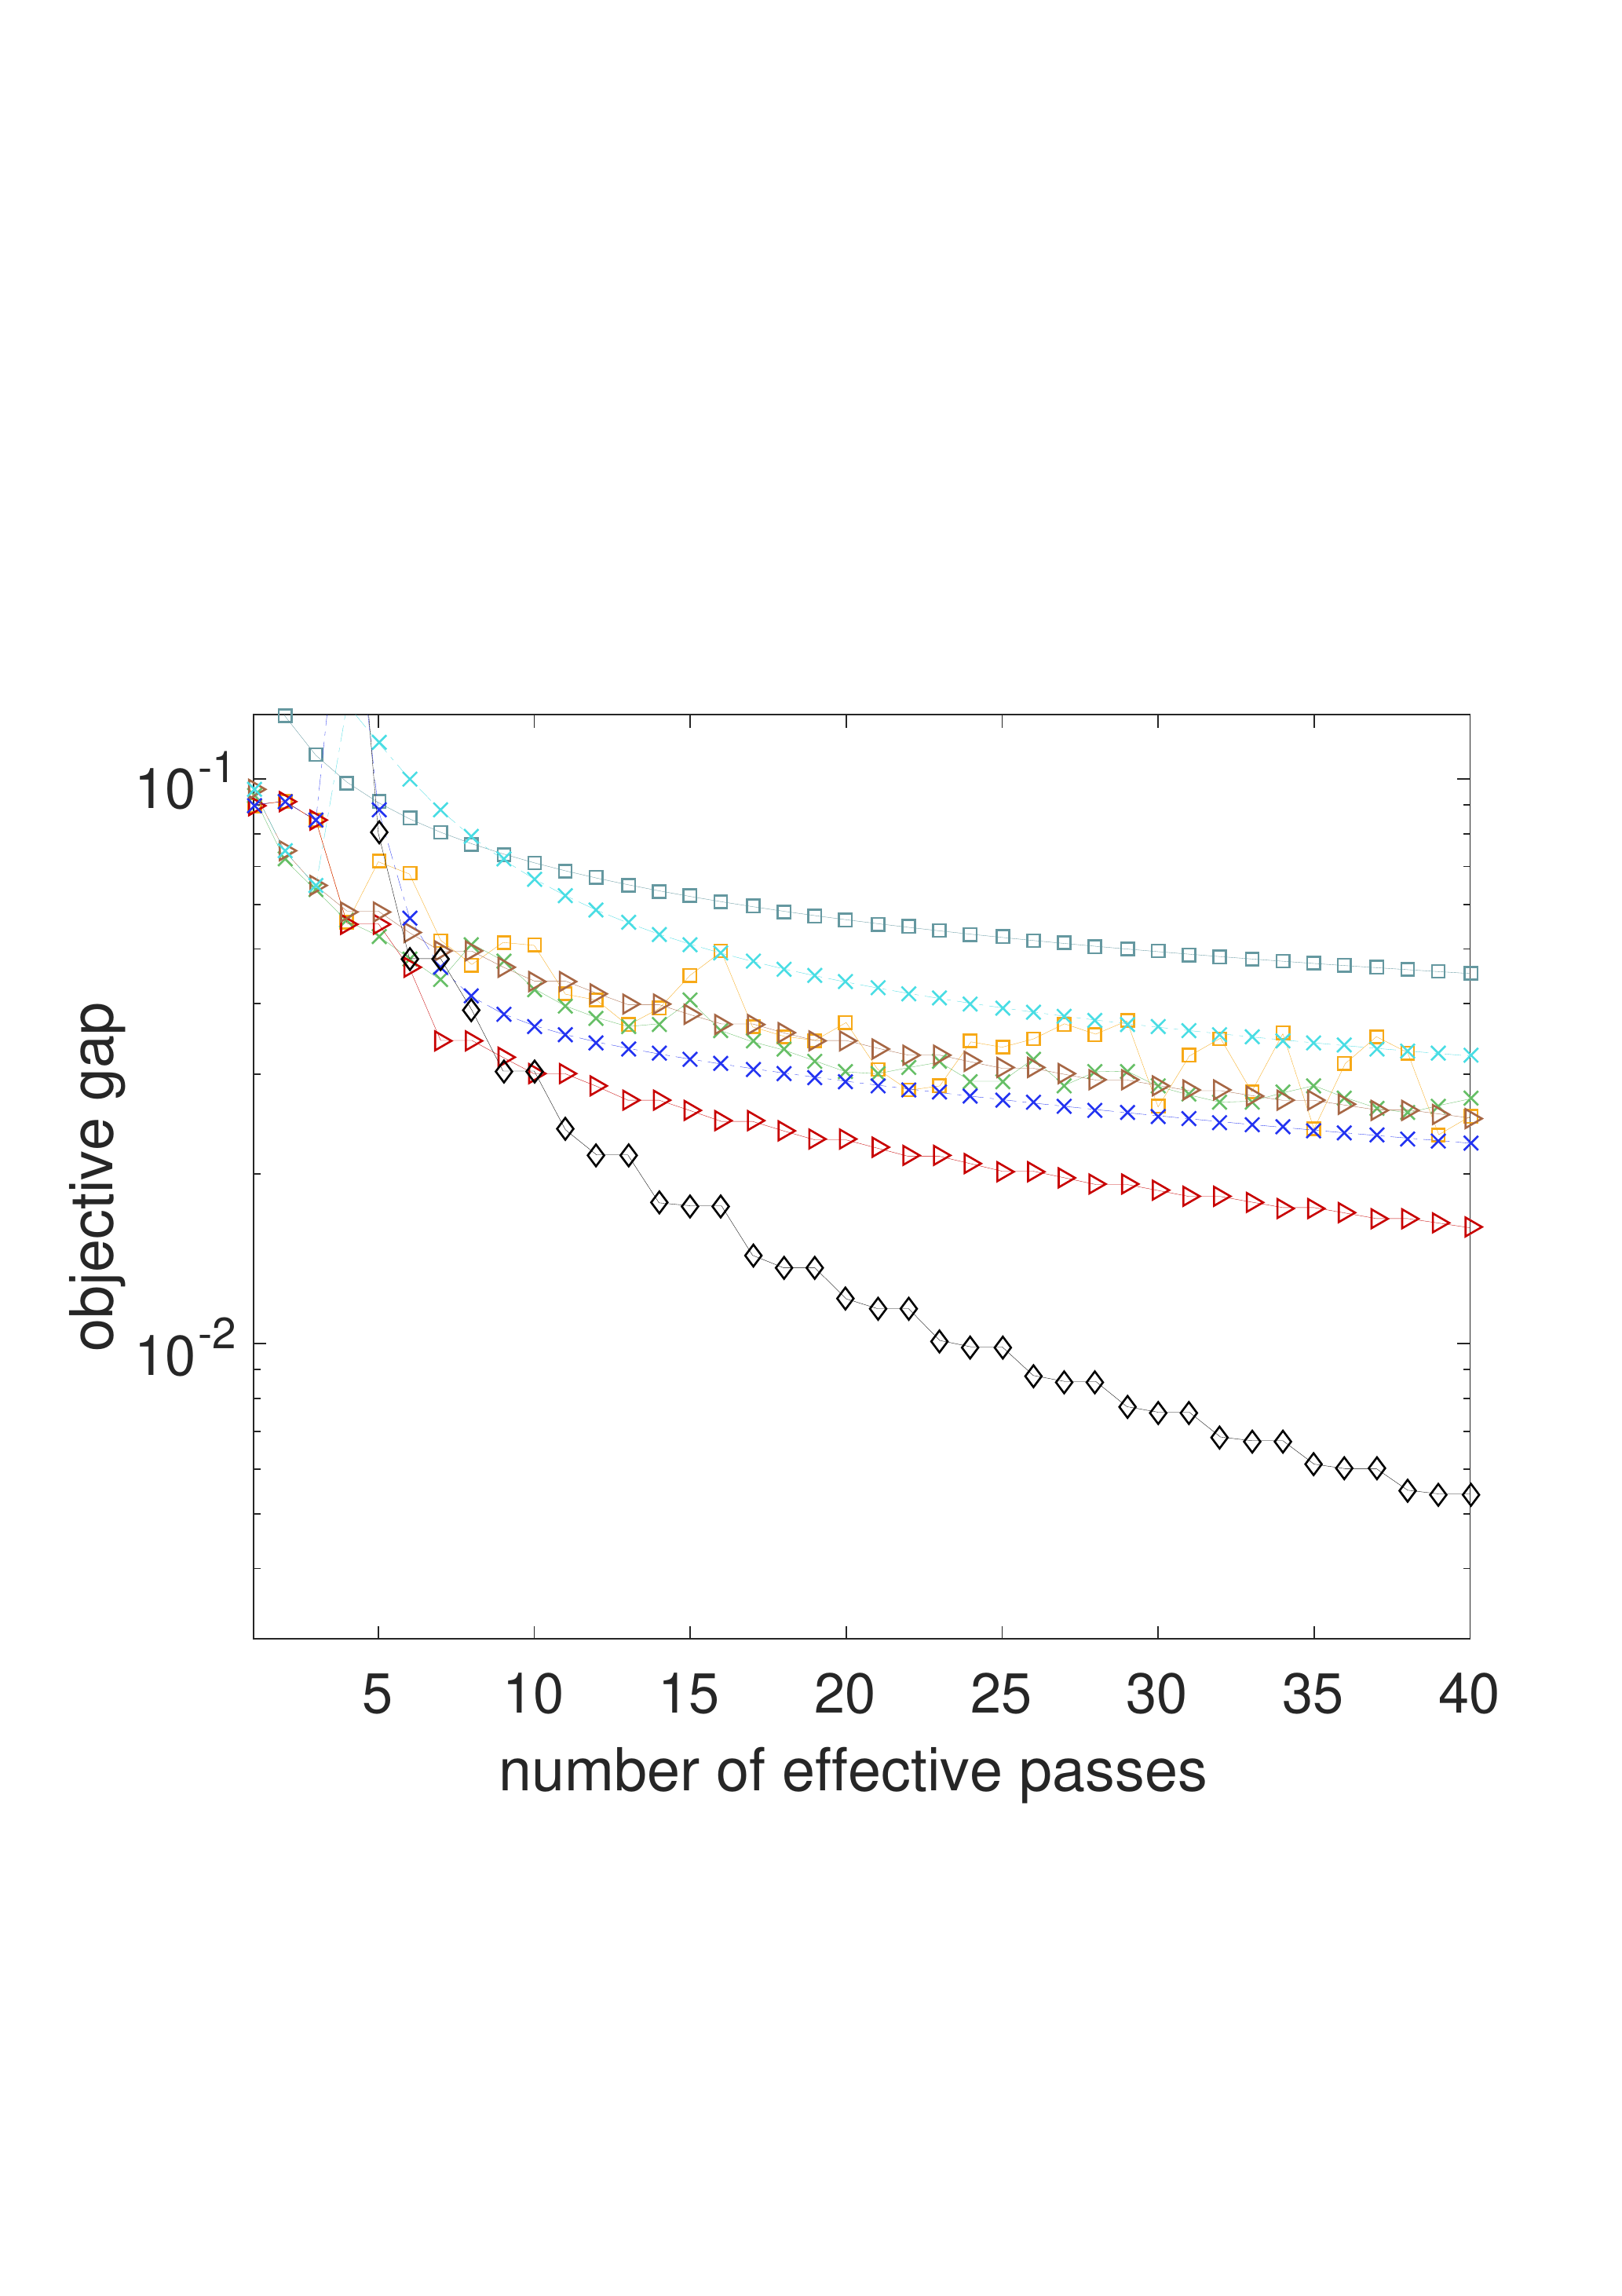}}
%	\hspace{-0.4in}   
	\subfigure{\hspace{-0.3in} 
		\label{fig:5} %% label for second subfigure 
		\includegraphics[width=1.1\linewidth]{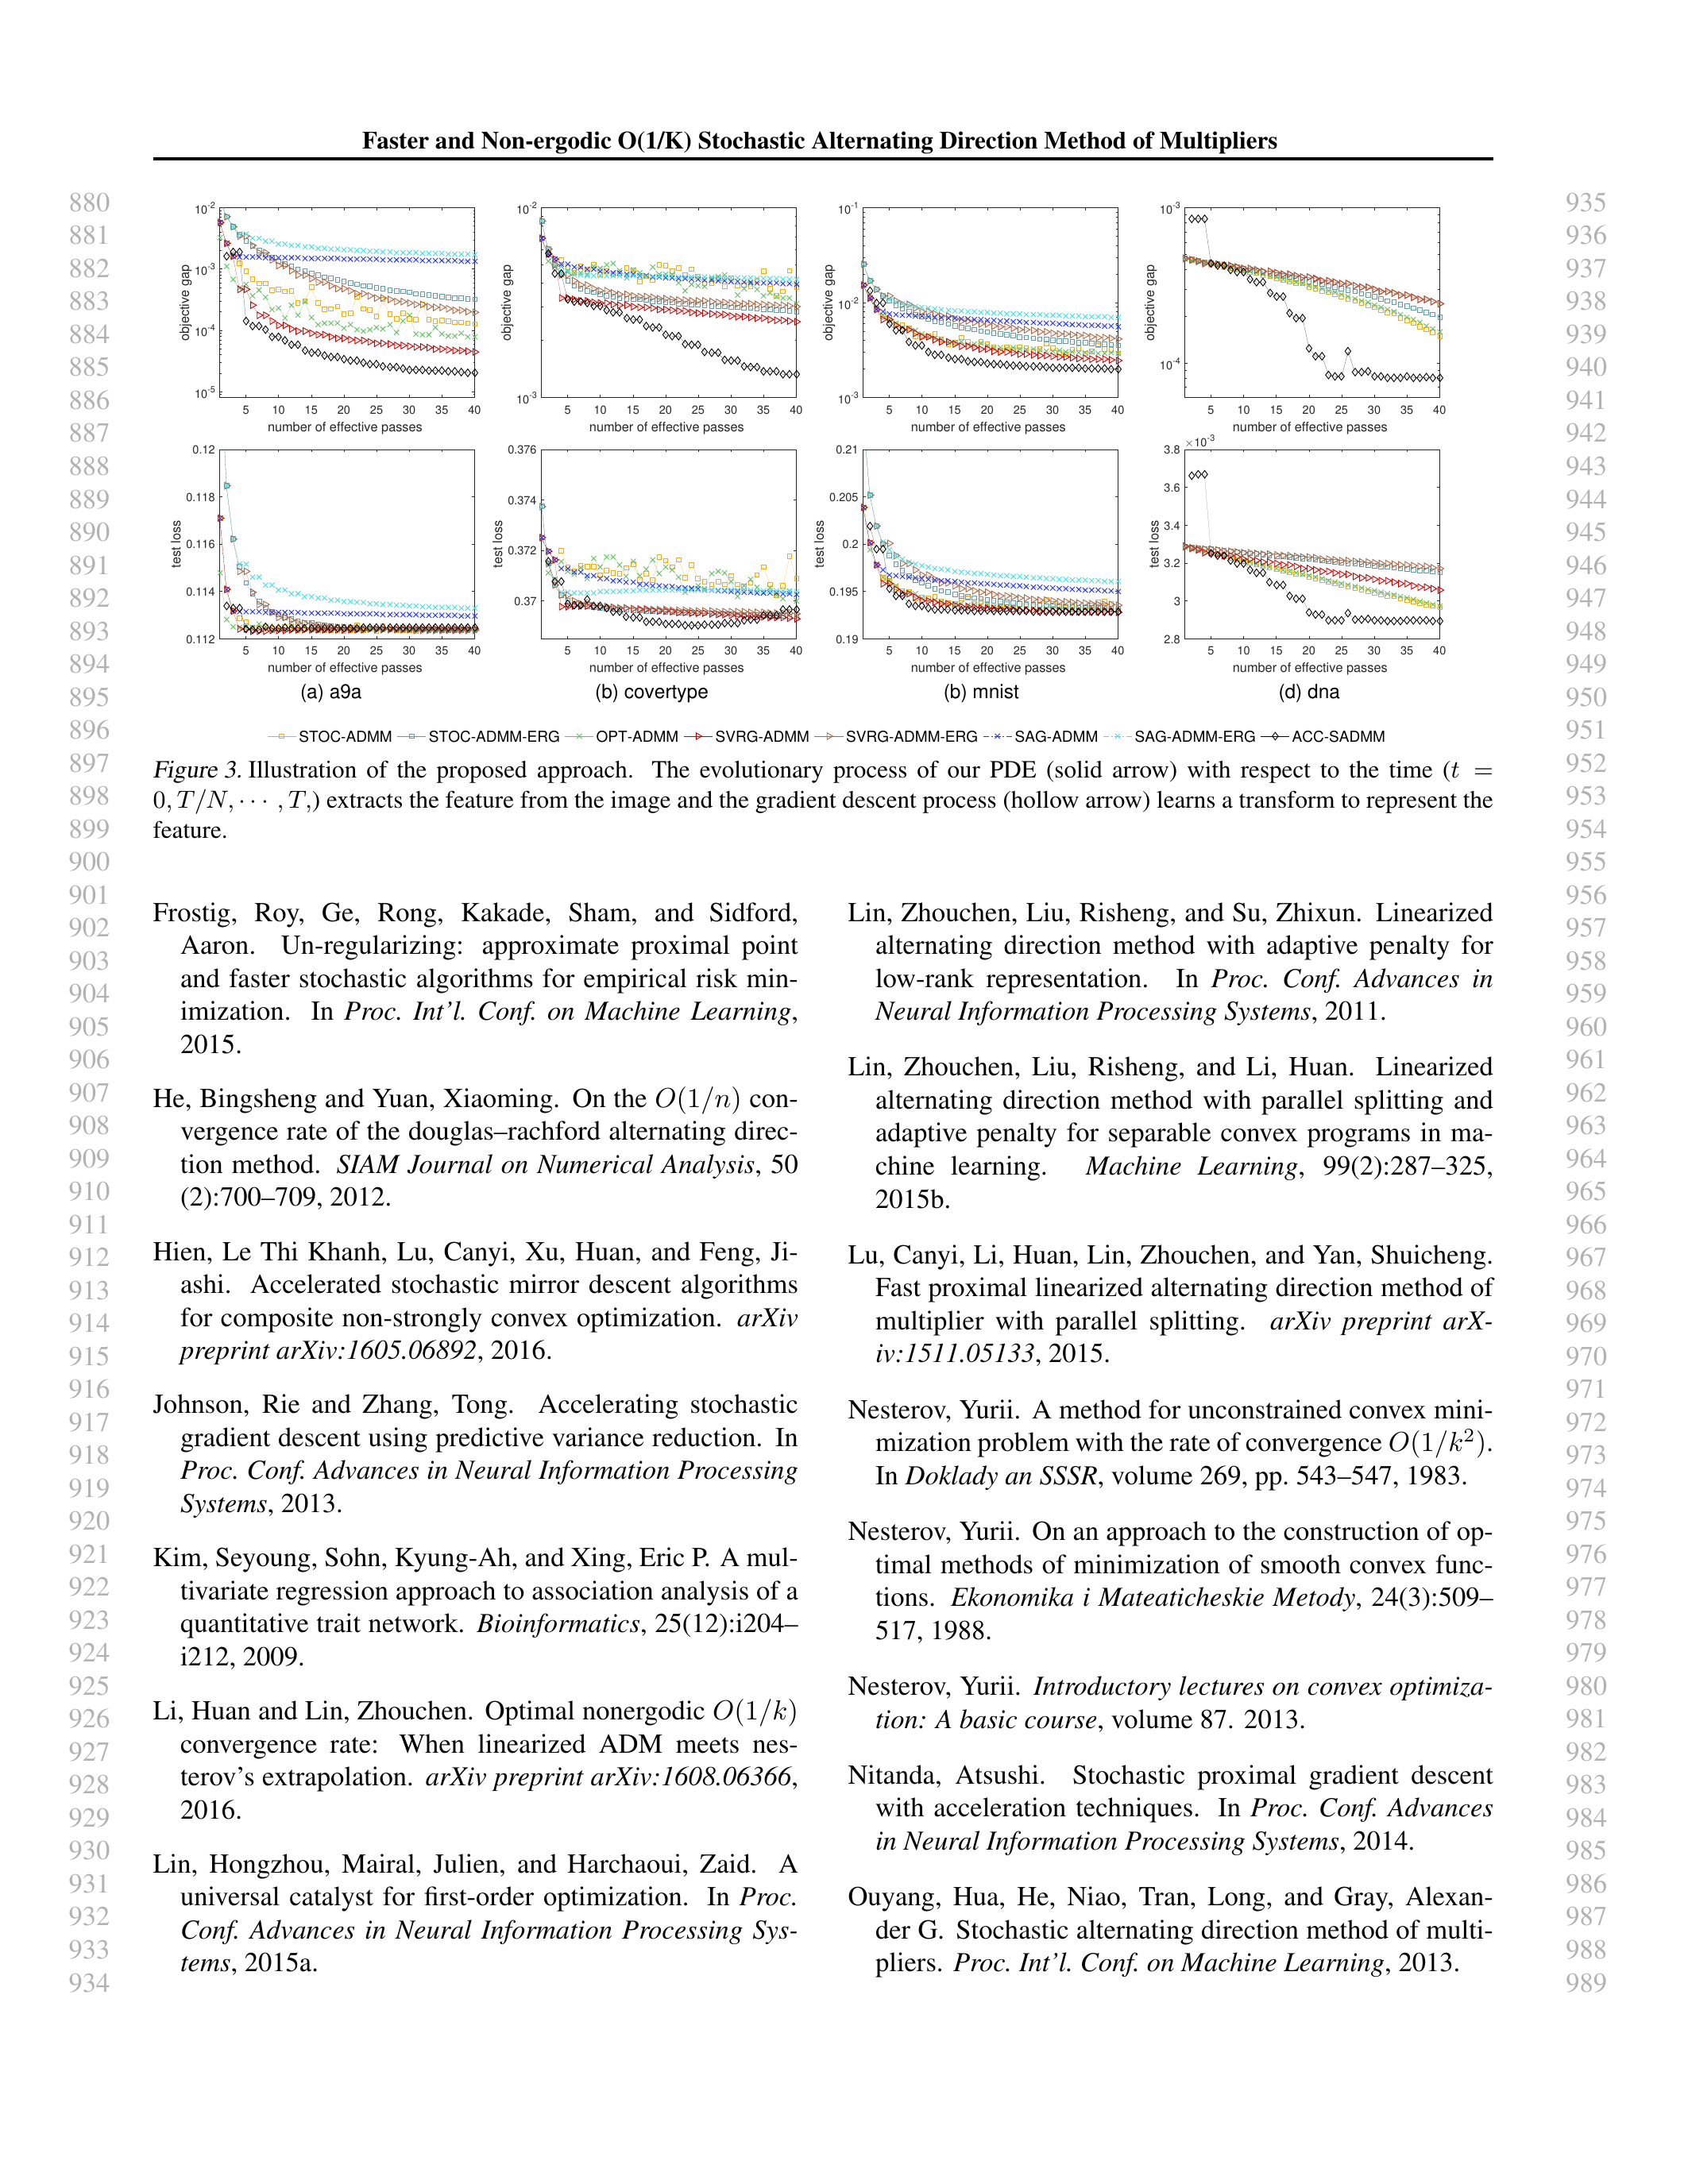}}  
	\vspace{-0.2in}     
	\caption{Experimental results of solving the  original Lasso (Eq.~(27)) and the Graph-Guided Fused Lasso problem (Eq.~(28)) on the a9a and mnist datasets with $L_2=0.01$.  }
	\label{experimentsss} %% label for entire figure 
\end{figure}

\begin{table}[!h]
	\small
	\centering
	\caption{Memory Costs for Storing Data on Different Datasets.}
	\begin{tabular} {|c |c |c|c|c|c|}\hline
		&a9a& covertype& mnist&dna&ImageNet\\\hline\hline
		STOC-ADMM&$2.31$KB&$1.69$KB&$123$KB&$25.0$KB&$62.5$MB\\\hline
		OPT-ADMM&$2.89$KB&$2.10$KB&$153$KB&$31.3$KB&$78.1$MB\\\hline
		SVRG-ADMM&$3.47$KB&$2.53$KB&$184$KB&$37.5$KB&$93.8$MB\\\hline
		SAG-ADMM&$82.9$MB&$0.23$GB&$3.50$GB&$28.6$GB&$38.2$TB\\\hline
		ACC-ADMM&$7.51$MB&$5.48$KB&$398$KB&$81.3$KB&$208$MB\\\hline
	\end{tabular}
	\label{memoryss}
\end{table}

\subsection{Description of Multitask Learning}
Multitask Learning experiment is performed on a 1000-class ImageNet dataset~\cite{russakovsky2015imagenet}. Since there is no parameter tuning issue, we use the validation set of ImageNet as the test set of the algorithms being compared. There are $1,281,167$ training images and the  validation set includes $50, 000$ images. 	$4096$ features are generated from the last fully connected layer of the convolutional  VGG-16 net~\cite{simonyan2014very}. We solve the  problem: $\min_{\X} l(X)+\mu_1\|\X\|_1+\mu_2\|\X\|_*$, where $l(\X)$ is the logistic loss. Like \cite{SVRG-ADMM}, we set $\mu_1=10^{-4}$ and $\mu_2=10^{-5}$. We set the mini-batchsize $b=2000$ since $\| \X \|_*$ should be solved through Singular Value Decomposition at each step. Our final test error is $30.9\%$ while  using the weight from the softmax layer of the original  VGG model~\cite{simonyan2014very}, the test error is  $32.4\%$.
